# Supplementary material for: Neyman-Pearson and equal opportunity: when efficiency meets fairness in classification
Source: arXiv:2310.01009 source file (2026-06-10)
Supplement: Supplementary file 1 [file npeo_appendix.pdf]

# Supplementary Material

## A NP-EO<sub>MP</sub> algorithms

Algorithm 1 (NP-EO<sub>OP</sub>) employs a “conservative” approach. Concretely, one pair of pivots, selected to ensure high-probability control on  $R_0^a$  and  $R_0^b$  simultaneously, serves as the lower bounds for the final thresholds. However, it could be suboptimal to control both  $R_0^a$  and  $R_0^b$ , as our goal is to control  $R_0$ ; indeed, it can induce unnecessarily small  $R_0$ , leading to large  $R_1$  and hurting the power of the classifier. To amend this, we can start from a sensitive-attribute-agnostic NP classifier, and then adjust the thresholds for both groups while maintaining the overall type I error control. This gives us a wider class of pivots (than in the NP-EO<sub>OP</sub> algorithm), and thus enables us to search for a more powerful classifier.

In our second and more general version of the NP-EO umbrella algorithm, we assume a slightly different sampling scheme for theoretical purposes. Denote by  $\mathcal{S}^y$  the set of  $(X, S)$  feature observations whose labels are  $y$ , where  $y \in \{0, 1\}$ . We assume that  $\mathcal{S}^0$  and  $\mathcal{S}^1$  are independent and the instances within each  $\mathcal{S}^y$  are i.i.d. Let  $\mathcal{S}^{y,s}$  be the set of  $X$  feature observations within  $\mathcal{S}^y$  whose sensitive attribute is  $s$ , where  $s \in \{a, b\}$ . Under this sampling scheme, we assume that  $n^y = |\mathcal{S}^y|$  is deterministic for  $y \in \{0, 1\}$ . Denote by  $n_s^y = |\mathcal{S}^{y,s}|$ ; then  $n_a^y$  and  $n_b^y$  are random, and  $n^y = n_a^y + n_b^y$ . Recall that we also denote  $p_{s|y} = \mathbb{P}(S = s \mid Y = y)$ . Each  $\mathcal{S}^{y,s}$  is split equally into  $\mathcal{S}_{\text{train}}^{y,s}$  and  $\mathcal{S}_{\text{left-out}}^{y,s}$ . Training of scoring function  $T$  (and thus  $T^a$  and  $T^b$ ) is the same as in Algorithm 1, and the scoring function  $T$  is again applied to all elements in  $\mathcal{S}_{\text{left-out}}^{y,s}$  to obtain the set of scores,  $\mathcal{T}^{y,s}$ , where  $y \in \{0, 1\}$  and  $s \in \{a, b\}$ . Similar to the approach outlined in Section 4.1, we first address the NP constraint. However, instead of two sensitive-attribute-specific thresholds, we start

with an intermediate classifier that has the same threshold for both groups:

$$\begin{aligned}\widehat{\phi}_*(X, S) &= \mathbb{I}\{T(X, S) > t_{(k_*)}^0\} \\ &= \mathbb{I}\{T^a(X) > t_{(k_*)}^0\} \mathbb{I}\{S = a\} + \mathbb{I}\{T^b(X) > t_{(k_*)}^0\} \mathbb{I}\{S = b\},\end{aligned}\quad (1)$$

where  $t_{(k_*)}^0$  is the  $(k_*)^{\text{th}}$  order statistic in  $\mathcal{T}^0 = \mathcal{T}^{0,a} \cup \mathcal{T}^{0,b}$  and  $k_*$  is selected by the NP umbrella algorithm on  $\mathcal{T}^0$ . This threshold selection guarantees that  $R_0(\widehat{\phi}_*)$  is controlled under  $\alpha$  with high probability. We will use  $\widehat{\phi}_*$  as a bridge. Concretely, if a classifier of the form in (6) admits the same empirical type I error on  $\mathcal{T}^0$  as  $\widehat{\phi}_*$ , their population-level type I errors should be close, and thus they can be both controlled under  $\alpha$  with probability close to  $1 - \alpha$ . One can see that  $\widehat{\phi}_*$  makes  $k_a^0 + k_b^0$  correct classifications on  $\mathcal{T}^0$ , where

$$k_a^0 = \sum_{j=1}^{n_a^0} \mathbb{I}\{t_j^{0,a} \leq t_{(k_*)}^0\} \quad \text{and} \quad k_b^0 = \sum_{j=1}^{n_b^0} \mathbb{I}\{t_j^{0,b} \leq t_{(k_*)}^0\}. \quad (2)$$

In fact, if any  $t_{(k_a)}^{0,a} \in \mathcal{T}_{0,a}$  and  $t_{(k_b)}^{0,b} \in \mathcal{T}_{0,b}$ , where  $k_a \in [n_a^0]$  and  $k_b \in [n_b^0]$ , are chosen as the thresholds for  $T^a$  and  $T^b$  respectively, then as long as  $k_a + k_b = k_a^0 + k_b^0$ , a classifier would have the same empirical type I error on  $\mathcal{T}^0$  as  $\widehat{\phi}_*$ . Thus, to respect the high-probability NP constraint, we might choose any pair of thresholds  $c_a, c_b$  such that  $c_a \geq t_{(k_a)}^{0,a}$  and  $c_b \geq t_{(k_b)}^{0,b}$ , where the pivots  $t_{(k_a)}^{0,a}$  and  $t_{(k_b)}^{0,b}$  satisfy  $k_a + k_b = k_a^0 + k_b^0$ . This larger collection of pivot pairs makes power improvement possible.

The next goal is to satisfy the high-probability EO constraint. Here, the steps and reasoning are similar to Algorithm 1. Let  $l_a(k_a)$  and  $l_b(k_b)$ , functions of  $k_a$  and  $k_b$ , be defined analogously to (9), with  $t_{(k_*)}^{0,a}$  and  $t_{(k_*)}^{0,b}$  replaced by  $t_{(k_a)}^{0,a}$  and  $t_{(k_b)}^{0,b}$ , respectively. Denote by  $\ell_a = \{l_a(1), \dots, l_a(n_a^0)\}$ , and  $\ell_b = \{l_b(1), \dots, l_b(n_b^0)\}$ . Similar to (9), as long as the two

thresholds  $c_a, c_b$  are selected from  $\left\{t_{(j)}^{1,a} : l_a(k_a) + 1 < j \leq l_a(k_a + 1)\right\}$  and  $\left\{t_{(j)}^{1,b} : l_b(k_b) + 1 < j \leq l_b(k_b + 1)\right\}$  respectively,<sup>1</sup> and  $k_a + k_b = k_a^0 + k_b^0$ , the high probability NP constraint can be respected.

Write

$$\mathbb{P}\left(|r_1^a(i) - r_1^b(j)| > \varepsilon\right) = \mathbb{E}_{s_r, \ell_a, \ell_b} \mathbb{P}\left(|r_1^a(i) - r_1^b(j)| > \varepsilon \mid s_r, \ell_a, \ell_b\right). \quad (3)$$

In the above,  $s_r$  stores the vector of the sensitive attributes associated with all instances in  $\mathcal{S}_{\text{left-out}}^{y,s}$ 's for  $y \in \{0, 1\}$  and  $s \in \{a, b\}$ . Recall that  $r_1^a(i)$  and  $r_1^b(j)$  are  $R_1^a$  and  $R_1^b$  if  $t_{(i)}^{1,a}$  and  $t_{(j)}^{1,b}$  are selected as thresholds. The next step is to approximate the conditional distributions of  $r_1^a(i)$  and  $r_1^b(j)$ .

The arguments here are similar to the ones in Section 4.1, and we will start from a similar motivating example. Let  $X$  and  $Y_1, Y_2, \dots, Y_n$  be continuous, independent, and identically distributed random variables. Now, let  $c_1, c_2, \dots, c_m$  be i.i.d. random variables that are independent of  $X, Y_1, \dots, Y_n$  and define  $l_i = \sum_{j=1}^n \mathbb{I}\{Y_j \leq c_i\}$  for  $i \in [m]$  and  $\ell = \{l_1, \dots, l_m\}$ . We will approximate the distribution of  $\mathbb{P}_X(X \leq Y_{(k)})$  conditional on  $\ell$ , which equals

$$\mathbb{P}_X(X \leq Y_{(k)}) \mid \ell \stackrel{d}{=} \begin{cases} B_{k, l_{(1)}-k+1} G_{c, \ell}^{(1)}, & k \leq l_{(1)}, \\ G_{c, \ell}^{(p)} + (G_{c, \ell}^{(p+1)} - G_{c, \ell}^{(p)}) B_{k-l_{(p)}, l_{(p+1)}-k+1}, & l_{(p)} < k \leq l_{(p+1)}, p \in [m-1], \\ G_{c, \ell}^{(m)} + (1 - G_{c, \ell}^{(m)}) B_{k-l_{(m)}, n-k+1}, & k > l_{(m)}, \end{cases}$$

where  $\stackrel{d}{=}$  means “equal in distribution”,  $B_{p,q} \sim \text{Beta}(p, q)$  and

---

<sup>1</sup> For simplicity of narrative,  $l_a(n_a^0 + 1)$  and  $l_a(n_a^0 + 1)$  are set to  $n_a^1$  and  $n_b^1$ , respectively.

$$G_{c,\ell} := \left[ G_{c,\ell}^{(1)}, G_{c,\ell}^{(2)}, \dots, G_{c,\ell}^{(m)} \right]^\top := [\mathbb{P}_{Y_1}(Y_1 \leq c_{(1)}), \mathbb{P}_{Y_1}(Y_1 \leq c_{(2)}), \dots, \mathbb{P}_{Y_1}(Y_1 \leq c_{(m)})]^\top \mid \ell.$$

Here,  $G_{c,\ell}$  and the Beta random variables are independent. The next step is to approximate the distribution of  $G_{c,\ell}$ . With a slight abuse of notation, denote  $c_{(0)} = -\infty, c_{(m+1)} = +\infty$  and  $l_{(0)} = 0, l_{(m+1)} = n$ . It suffices to consider the joint distribution of the quantity

$$\Delta G_c \mid \Delta \ell := [\mathbb{P}_{Y_1}(c_{(j-1)} < Y_1 \leq c_{(j)}), j \in [m+1]]^\top \mid [l_{(i)} - l_{(i-1)}, i \in [m]]^\top.$$

For fixed  $c_j$ ,  $\Delta G_c = [\mathbb{P}_{Y_1}(c_{(j-1)} < Y_1 \leq c_{(j)}), j \in [m+1]]^\top$  can be viewed as the vector of probabilities for a multinomial distribution, and  $\Delta \ell = [l_{(i)} - l_{(i-1)}, i \in [m+1]]^\top$  is a multinomial random variable of size  $n$  generated from this distribution. Then, the maximum likelihood estimator for  $\Delta G_c$  is  $\frac{\Delta \ell}{n}$ . Therefore, when  $c_j$  is random for  $j \in [m]$ , the distribution of  $\Delta G_c \mid \Delta \ell$  is the posterior distribution of  $\Delta G_c$  given  $\Delta \ell$ , and thus, by invoking Bernstein-von Mises theorem again, is “close to” Gaussian centered at  $\frac{\Delta \ell}{n}$  with covariance matrix  $\Sigma$  where

$$\Sigma_{i,j} = \begin{cases} \frac{1}{n} \mathbb{P}_{Y_1}(c_{(j-1)} < Y_1 \leq c_{(j)}) (1 - \mathbb{P}_{Y_1}(c_{(j-1)} < Y_1 \leq c_{(j)})), & i = j, \\ -\frac{1}{n} \mathbb{P}_{Y_1}(c_{(i-1)} < Y_1 \leq c_{(i)}) \mathbb{P}_{Y_1}(c_{(j-1)} < Y_1 \leq c_{(j)}), & i \neq j. \end{cases}$$

Furthermore, we can use  $(l_{(j)} - l_{(j-1)})/n$  to replace  $\mathbb{P}_{Y_1}(c_{(j-1)} < Y_1 \leq c_{(j)})$  and obtain an estimated covariance matrix  $\hat{\Sigma}$ . Thus, the estimation of  $\mathbb{P}_X(X \leq Y_{(k)}) \mid \ell$  is finished.

Despite being lengthy, it is actually straightforward to relate this example with the problem in this section. Recall that in view of (3), the goal is to approximate the distribution of  $(r_1^a(i) \mid \ell_a)$ . Note that conditional on scoring function  $T^a$  and  $s_r$ , the scores

$t_1^{1,a}, t_2^{1,a}, \dots, t_{n_a^1}^{1,a}$  are i.i.d. random variables, and  $t_1^{0,a}, t_2^{0,a}, \dots, t_{n_a^0}^{0,a}$  are also i.i.d. random variables. Furthermore, the two groups of random variables are mutually independent. Moreover,  $r_1^a(i) = \mathbb{P}_{t^{1,a}}(t_1^{1,a} \leq t_{(i)}^{1,a})$  and  $l_a(j) = \sum_{h=1}^{n_a^1} \mathbb{1}\{t_h^{1,a} \leq t_{(j)}^{0,a}\}$  for every  $i \in [n_a^1]$  and  $j \in [n_a^0]$ . Therefore, the problem setting is in line with the previous motivating example, and thus, the distribution of  $r_1^a(i) \mid \ell_a$  can be approximated in the same way. And the same procedure can be applied to the  $S = b$  component. To conclude, we select  $i$  and  $j$  such that

$$\mathbb{P}\left(\left|\tilde{F}^{1,a}(i) - \tilde{F}^{1,b}(j)\right| > \varepsilon\right) \leq \gamma, \quad (4)$$

where

$$\tilde{F}^{1,a}(i) \stackrel{d}{=} \begin{cases} B_{k, l_a(1)-k+1} \tilde{G}_1^{1,a}, & k \leq l_a(1), \\ \tilde{G}_p^{1,a} + \left(\tilde{G}_{p+1}^{1,a} - \tilde{G}_p^{1,a}\right) B_{k-l_a(p), l_a(p+1)-k+1}, & l_a(p) < k \leq l_a(p+1), p \in [n_a^0 - 1], \\ \tilde{G}_{n_a^0}^{1,a} + (1 - \tilde{G}_{n_a^0}^{1,a}) B_{k-l_a(n_a^0), n_a^1-k+1}, & k > l_a(n_a^0), \end{cases}$$

and  $\tilde{G}^{1,a} = [G_1^{1,a}, \dots, G_{n_a^0}^{1,a}]^\top$  is a Gaussian vector with mean  $[l_a(1)/n_a^1, \dots, l_a(n_a^0)/n_a^1]^\top$  and covariance matrix

$$\begin{bmatrix} \frac{(d_a(1)/n_a^1)(1-d_a(1)/n_a^1)}{n_a^1} & -\frac{(d_a(1)/n_a^1)(d_a(2)/n_a^1)}{n_a^1} & \dots & -\frac{(d_a(1)/n_a^1)(d_a(n_a^0+1)/n_a^1)}{n_a^1} \\ -\frac{(d_a(2)/n_a^1)(d_a(1)/n_a^1)}{n_a^1} & \frac{(d_a(2)/n_a^1)(1-d_a(2)/n_a^1)}{n_a^1} & \dots & -\frac{(d_a(2)/n_a^1)(d_a(n_a^0+1)/n_a^1)}{n_a^1} \\ \vdots & \vdots & \ddots & \vdots \\ -\frac{(d_a(n_a^1+1)/n_a^1)(d_a(1)/n_a^1)}{n_a^1} & -\frac{(d_a(n_a^1+1)/n_a^1)(d_a(2)/n_a^1)}{n_a^1} & \dots & \frac{(d_a(n_a^0+1)/n_a^1)(1-d_a(n_a^0+1)/n_a^1)}{n_a^1} \end{bmatrix}.$$

Here,

$$d_a(k) = \begin{cases} l_a(1), & k = 1, \\ l_a(k+1) - l_a(k), & k = 2, 3, \dots, n_a^0 - 1, \\ n_a^1 - l_a(n_a^0), & k = n_a^0. \end{cases}$$

Moreover,  $\tilde{F}^{1,b}(j)$  is defined analogously. Details of this approximation can be found in Algorithm 4 in the Appendix. Next, one pair of  $i$  and  $j$  needs to be selected among all possible pairs satisfying (4). In Algorithm 1, we traverse all feasible pairs of  $i$  and  $j$  and choose one that minimizes the empirical type II error. It was computationally feasible because only  $i, j$  such that  $t_{(i)}^{1,a} > t_{(k_*^0,a)}^{0,a}$  and  $t_{(j)}^{1,b} > t_{(k_*^0,b)}^{0,b}$  were considered. However, our generalized algorithm NP-EO<sub>MP</sub> has multiple pairs of pivots, and it could be time-consuming to do the same. Therefore, we adopt the following heuristics:

1. Compute  $t_{(k_*)}^0$  by the NP umbrella algorithm. Then, select  $k_a^0$  and  $k_b^0$  by (2) and set  $k_a = k_a^0$  and  $k_b = k_b^0$ .
2. Given  $k_a$  and  $k_b$ , set  $i = l_a(k_a) + 1$  and  $j = l_b(k_b) + 1$ , i.e.,  $i$  is such that  $t_{(i)}^{1,a}$  is the smallest element in  $\mathcal{T}^{1,a}$  larger than  $t_{(k_a)}^{0,a}$ , and  $j$  is selected analogously.
3. Apply Algorithm 4 to  $i, j$ <sup>2</sup> to calculate the approximate one-sided EO violation rates  $\mathbb{P}(\tilde{F}^{1,a}(i) - \tilde{F}^{1,b}(j) \geq \varepsilon)$  and  $\mathbb{P}(\tilde{F}^{1,b}(j) - \tilde{F}^{1,a}(i) \geq \varepsilon)$ . If the former approximation is larger than  $\gamma$ , i.e.,  $\tilde{F}^{1,a}(i)$  is too large, increase  $k_b$  by 1 and decrease  $k_a$  by 1. If the latter approximation is larger than  $\gamma$ , increase  $k_a$  by 1 and decrease  $k_b$  by 1.
4. Repeat Steps (2) - (3) until the approximate value  $\mathbb{P}(|\tilde{F}^{1,a}(i) - \tilde{F}^{1,b}(j)| \geq \varepsilon)$  is smaller

---

<sup>2</sup>  $i, j$  are inputs as  $k(a)$  and  $k(b)$  in Algorithm 4.

than or equal to  $\gamma$ , then use  $t_{(i)}^{1,a}$  and  $t_{(j)}^{1,b}$  as thresholds.<sup>3</sup>

Let us briefly discuss the above procedure. After key quantities  $t_{(k_*)}^0$ ,  $k_a^0$ , and  $k_b^0$  are determined,  $k_a$  and  $k_b$  are set to  $k_a^0$  and  $k_b^0$ , respectively, in Step (1). In Step (2) and (3), an iterative method is used to find  $i$  and  $j$  that satisfy (4). For a pair of  $k_a$  and  $k_b$ , we only look at  $i$  and  $j$  such that  $t_{(i)}^{1,a}$  and  $t_{(j)}^{1,b}$  are the smallest elements in  $\mathcal{T}^{1,a}$  and  $\mathcal{T}^{1,b}$  that are larger than  $t_{(k_a)}^{0,a}$  and  $t_{(k_b)}^{0,b}$ , respectively. If this pair of  $i$  and  $j$  fails to satisfy (4), we adjust  $k_a$  and  $k_b$ , and then update  $i$  and  $j$  accordingly. For example, if  $\mathbb{P}(\tilde{F}^{1,a}(i) - \tilde{F}^{1,b}(j) \geq \varepsilon) > \gamma$ , i.e.,  $\tilde{F}^{1,a}(i)$  is too large and  $\tilde{F}^{1,b}(j)$  is too small, we decrease  $k_a$  by 1 and increase  $k_b$  by 1, so that  $k_a + k_b = k_a^0 + k_b^0$  and thus high-probability NP constraint is respected. After  $k_a$  and  $k_b$  are updated,  $i$  and  $j$  are selected in the same way described above. This updating procedure can be done iteratively until (4) is reached. Then, the scores  $t_{(i)}^{1,a}$  and  $t_{(j)}^{1,b}$  are selected as the thresholds of the resulting classifier.

This more general version of NP-EO umbrella algorithm is summarized as Algorithm 2. Instead of using only one pair of pivots in Algorithm 1, Algorithm 2 uses multiple pairs. Concretely, the two pivots  $t_{(k_a)}^{0,a}$  and  $t_{(k_b)}^{0,b}$  can be increased or decreased based on their resulting one-sided type II error disparities. Algorithm 1 controls  $R_0^a$  and  $R_0^b$  simultaneously to achieve the high-probability NP constraint. Algorithm 2, however, relieves the control on one of them but uses the empirical type I errors as a bridge to have an “approximate control” on the population-level type I error. This increases the risk of failing the exact probability target of type I error control. However, the advantage of this less conservative approach is obvious: lowering the pivot on one side allows a higher classification power. Indeed, numerical evidence from Section 5.1 suggests that Algorithm 2 has a lower type II

---

<sup>3</sup> There are exceptions where Step (4) cannot be achieved by repeating Steps (2) - (3). However, these can be handled subtly by adjusting  $i$  and  $j$ . Details are included in Algorithm 5 in the Appendix.

---

**Algorithm 2:** NP-EO<sub>MP</sub> umbrella algorithm [“MP” means Multiple (Pairs of) Pivots]

---

**Input** :  $\mathcal{S}^{y,s}$ :  $X$  observations whose label  $y \in \{0, 1\}$  and sensitive attribute  $s \in \{a, b\}$   
 $\alpha$ : upper bound for type I error  
 $\delta$ : type I error violation rate target  
 $\varepsilon$ : upper bound for the type II error disparity  
 $\gamma$ : type II error disparity violation rate target

- 1  $\mathcal{S}_{\text{train}}^{y,s}, \mathcal{S}_{\text{left-out}}^{y,s} \leftarrow$  random split on  $\mathcal{S}^{y,s}$  for  $y \in \{0, 1\}$  and  $s \in \{a, b\}$
- 2  $\mathcal{S}_{\text{train}} \leftarrow \mathcal{S}_{\text{train}}^{0,a} \cup \mathcal{S}_{\text{train}}^{0,b} \cup \mathcal{S}_{\text{train}}^{1,a} \cup \mathcal{S}_{\text{train}}^{1,b}$
- 3  $T \leftarrow$  base classification algorithm( $\mathcal{S}_{\text{train}}$ ) ; //  $T(\cdot, \cdot) : \mathcal{X} \times \{a, b\} \mapsto \mathbb{R}$
- 4  $T^s(\cdot) \leftarrow T(\cdot, s)$  for  $s \in \{a, b\}$
- 5  $\mathcal{T}^{y,s} \leftarrow T^s(\mathcal{S}_{\text{left-out}}^{y,s})$  for  $y \in \{0, 1\}$  and  $s \in \{a, b\}$
- 6  $n_s^y \leftarrow |\mathcal{T}^{y,s}|$  for  $y \in \{0, 1\}$  and  $s \in \{a, b\}$
- 7  $\mathcal{T}^0 = \mathcal{T}^{0,a} \cup \mathcal{T}^{0,b} = \{t_{(1)}^0, t_{(2)}^0, \dots, t_{(n^0)}^0\}$ , where  $n^0 = n_a^0 + n_b^0$
- 8  $\mathcal{T}^{y,s} = \{t_{(1)}^{y,s}, t_{(2)}^{y,s}, \dots, t_{(n_s^y)}^{y,s}\}$  for  $y \in \{0, 1\}$  and  $s \in \{a, b\}$
- 9  $k_* \leftarrow$  the NP umbrella algorithm( $n^0, \alpha, \delta$ )
- 10  $\{l_s(1), \dots, l_s(n_s^0)\} \leftarrow \left\{ \sum_{j=1}^{n_s^1} \mathbb{I}\{t_j^{1,s} \leq t_{(1)}^{1,s}\}, \dots, \sum_{j=1}^{n_s^1} \mathbb{I}\{t_j^{1,s} \leq t_{(n_s^1)}^{1,s}\} \right\}$  for  $s \in \{a, b\}$
- 11  $k_s \leftarrow k_s^0 \leftarrow \sum_{j=1}^{n_s^0} \mathbb{I}\{t_j^{0,s} \leq t_{(k_*)}^{0,s}\}$  for  $s \in \{a, b\}$
- 12  $(k_a^*, k_b^*) \leftarrow$  Order selection algorithm( $k_s, n_s^y, l_s(1), \dots, l_s(n_s^0), \varepsilon, \gamma$ ) for  $s \in \{a, b\}$

**Output:**  $\hat{\phi}^{**}(X, S) = \mathbb{I}\{T^a(X) > t_{(k_a^*)}^{1,a}\} \cdot \mathbb{I}\{S = a\} + \mathbb{I}\{T^b(X) > t_{(k_b^*)}^{1,b}\} \cdot \mathbb{I}\{S = b\}$

---

error compared to Algorithm 1 and a higher type I error. Furthermore, both algorithms satisfy high-probability NP and EO constraints. Same as in Section 4.1, in theory, there could be exceptions that no  $(i, j)$  satisfies (4). However, we have not met this exception in data analysis.

The theoretical guarantee for Algorithm 2 is presented in Theorem 3. Since the empirical type I errors are used as a bridge to link the population-level type I errors for different pairs of pivots, a concentration of empirical type I errors towards population-level type I error is needed. Thus, in the following theoretical result, we allow an  $\eta$ -error between empirical and population-level type I errors. That is, the target probability for type I error control will be set at  $\alpha - \eta$  where  $\eta$  is a small number compared with  $\alpha$ . However, this is not needed in the numerical implementation of Algorithm 2.

## B Preliminaries

### B.1 NP umbrella algorithm

The NP umbrella algorithm developed in Tong et al. [2018] adapts all scoring-type classification methods (e.g., logistic regression, random forest, neural nets) so that the resulting classifiers have the type I error bounded from above by a user-specified level  $\alpha$  with pre-specified high probability  $1 - \delta$ . In this section, we provide a description of NP umbrella algorithm (without the protected attributes) for readers' convenience.

Decompose the observations  $\mathcal{S}$  by  $\mathcal{S} = \mathcal{S}^0 \cup \mathcal{S}^1$ , where  $\mathcal{S}^0$  is the set of all instances of class 0 and  $\mathcal{S}^1$  is the set of instances of class 1. Assume that the observations in  $\mathcal{S}^0$  and  $\mathcal{S}^1$  are independent. Split  $\mathcal{S}^0$  randomly into two parts  $\mathcal{S}_{\text{train}}^0$  and  $\mathcal{S}_{\text{left-out}}^0$ . The sets  $\mathcal{S}^1$  and  $\mathcal{S}_{\text{train}}^0$  are combined to train a scoring function  $T$  (e.g., sigmoid function in logistic regression). Apply  $T$  to all instances of  $\mathcal{S}_{\text{left-out}}^0 = \{X_1^0, \dots, X_n^0\}$  and denote  $\{t_1, \dots, t_n\} := \{T(X_1^0), \dots, T(X_n^0)\}$ . Then we have

**Theorem S.1.** *Denote  $\mathcal{T} = \{t_{(1)}, t_{(2)}, \dots, t_{(n)}\}$  where  $t_{(1)} \leq t_{(2)} \leq \dots \leq t_{(n)}$ . Then, for any  $\alpha \in (0, 1)$ ,*

$$\mathbb{P} \left( \mathbb{P}_{\mathcal{S}} (T(X) > t_{(k)} \mid Y = 0) > \alpha \right) \leq \sum_{j=k}^n \binom{n}{j} \alpha^{n-j} (1 - \alpha)^j,$$

where the outer  $\mathbb{P}$  is taken with respect to the randomness of  $\mathcal{S}$ .

Hence, the classifier  $\phi(X) = \mathbb{I}\{T(X) > t_{(k^*)}\}$  is able to control the type I error under  $\alpha$  with probability at least  $1 - \delta$ , where  $k^*$  is the smallest integer among  $\{1, 2, \dots, n\}$  such

that

$$\sum_{j=k}^n \binom{n}{j} \alpha^{n-j} (1-\alpha)^j \leq \delta.$$

The smallest  $k$  was chosen because we want to achieve a type II error as small as possible.

## B.2 Bernstein-von Mises Theorem

Let  $\{P_\theta, \theta \in \Theta\}$  be a family of distributions where  $\Theta$  is a measurable set. For every  $\theta \in \Theta$ ,  $P_\theta$  has a density function  $p_\theta$  with respect to a common measure  $\mu$ . Moreover, a prior distribution whose density  $\pi$  is defined on  $\Theta$ . Furthermore, let  $X_1, X_2, \dots, X_n$  be i.i.d. random variables with distribution  $P_{\theta_0}$  for some  $\theta_0 \in \Theta$ . Then, the posterior distribution  $\Pi(\cdot|X_1, \dots, X_n)$  is defined as follows. By any measurable set  $B \subset \Theta$ ,

$$\Pi(B|X_1, \dots, X_n) = \frac{\int_B \prod_{j=1}^n p_\theta(X_j) \pi(\theta) d\theta}{\int_\Theta \prod_{j=1}^n p_\theta(X_j) \pi(\theta) d\theta}.$$

Next, define  $\hat{\theta}_n = \hat{\theta}_n(X_1, X_2, \dots, X_n)$  be the maximum likelihood estimator of  $\theta_0$ , i.e.,

$$\hat{\theta}_n = \operatorname{argmax}_{\theta \in \Theta} \prod_{j=1}^n p_\theta(X_j)$$

Then, the famous Bernstein-von Mises theorem links the Bayesian and frequentists' points of view. Many versions of conditions for Bernstein-von Mises can be found in the literature.

We will adopt the version in Ghosh and Ramamoorthi [2011].

1.  $\{x : p_\theta(x) > 0\}$  is the same for all  $\theta \in \Theta$ .
2.  $L(\theta, x) = \log p_\theta(x)$  is thrice differentiable with respect to  $\theta$  in  $(\theta_0 - a, \theta_0 + a)$  for some

small  $a$ . Denote  $L'(\theta), L''(\theta)$  and  $L'''(\theta)$  to be the first, second and third derivative, respectively. Then, assume  $E_{\theta_0} L'(\theta_0), E_{\theta_0} L''(\theta_0)$  to be finite and

$$\sup_{\theta \in (\theta_0 - a, \theta_0 + a)} |L'''(\theta)| < M(x),$$

and  $E_{\theta_0} M < \infty$ , where  $E_{\theta_0}$  is the expectation taken with respect to the measure  $P_{\theta_0}$ .

3.

$$E_{\theta_0} L'(\theta_0) = \partial_{\theta} E_{\theta_0} L(\theta_0) = 0 \text{ and } E_{\theta_0} L''(\theta_0) = -E_{\theta_0} (L'(\theta_0))^2 < 0.$$

4. For any  $\delta > 0$ , there exists an  $\varepsilon > 0$  such that

$$P_{\theta_0} \left( \sup_{|\theta - \theta_0| > \delta} \frac{1}{n} (L_n(\theta) - L_n(\theta_0)) \leq -\varepsilon \right) \rightarrow 1,$$

where  $L_n(\theta) = \sum_{j=1}^n L(\theta, X_j)$  for any  $\theta$ .

5. The prior  $\pi$  is continuous and positive at  $\theta_0$ .

**Theorem S.2.** *Under the aforementioned conditions,*

$$\left\| \Pi(\cdot | X_1, \dots, X_n) - \mathcal{N} \left( \hat{\theta}_n, \frac{1}{n} i^{-1}(\theta_0) \right) \right\|_{TV} \rightarrow 0,$$

*in probability. Here,  $i(\theta) = E_{\theta_0} (L'(\theta_0))^2$  is the Fisher information of  $\theta$  and  $\|\cdot\|_{TV}$  is the total variation distance.*

### B.3 Generalized Neyman-Pearson Lemma

For the readers' convenience, we reproduce the generalized Neyman-Pearson Lemma. This version is Theorem 3.6.1 from the textbook "Testing Statistical Hypotheses" (3rd edition) [Lehmann and Ramano, 2005].

**Theorem S.3.** *Let  $f_1, \dots, f_{m+1}$  be real-valued functions defined on a Euclidean space  $\mathcal{X}$  and integrable  $\mu$ , and suppose that for given constants  $c_1, \dots, c_m$ , there exists a critical function  $\phi$  satisfying*

$$\int \phi f_i d\mu = c_i, \quad i = 1, \dots, m. \quad (5)$$

*Let  $\mathcal{C}$  be the class of critical functions  $\phi$  for which (5) holds.*

*(i) Among all members of  $\mathcal{C}$ , there exists one that maximizes*

$$\int \phi f_{m+1} d\mu.$$

*(ii) A sufficient condition for a member of  $\mathcal{C}$  to maximize*

$$\int \phi f_{m+1} d\mu$$

*is the existence of constants  $k_1, \dots, k_m$  such that*

$$\begin{aligned} \phi(x) &= 1 & \text{when} & & f_{m+1}(x) > \sum_{i=1}^m k_i f_i(x), \\ \phi(x) &= 0 & \text{when} & & f_{m+1}(x) < \sum_{i=1}^m k_i f_i(x). \end{aligned} \quad (6)$$

(iii) If a member of  $\mathcal{C}$  satisfies (6) with  $k_1, \dots, k_m \geq 0$ , then it maximizes

$$\int \phi f_{m+1} d\mu$$

among all critical functions satisfying

$$\int \phi f_i d\mu \leq c_i, \quad i = 1, \dots, m.$$

(iv) The set  $M$  of points in  $m$ -dimensional space whose coordinates are

$$\left( \int \phi f_1 d\mu, \dots, \int \phi f_m d\mu \right)$$

for some critical function  $\phi$  is convex and closed. If  $(c_1, \dots, c_m)$  is an inner point of  $M$ , then there exists constants  $k_1, \dots, k_m$  and a test  $\phi$  satisfying (5) and (6), and a necessary condition for a member of  $\mathcal{C}$  to maximize

$$\int \phi f_{m+1} d\mu$$

is that (6) holds a.e.  $\mu$ .

## B.4 More discussion on choices of $\alpha$ and $\varepsilon$

While perfect fairness offers clear standards and strong guarantees, it often comes at the cost of significant loss in predictive accuracy [Denis et al., 2024]. Therefore, approximate fairness is of great practical value and widely adopted [Celis et al., 2019, Denis et al.,

2024], which aligns with the focus of our work. In this context, practitioners can adjust their tolerance levels for fairness; however, this may result in less equitable outcomes, highlighting the need for guidance on parameter selection. Although there is no one-size-fits-all rule, we aim to provide some literature and insights regarding these parameters.

For instance, concerning the fairness constraint ( $\varepsilon$ ), disparate impact is rooted in the 80% rule established by the U.S. Equal Employment Opportunity Commission [Commission et al., 1979, Menon and Williamson, 2018]. Similarly, a tolerance level of around 20% is commonly accepted in various fields [Denis et al., 2024, Holzer and Neumark, 2000, Collins, 2007]. A parallel argument can be made regarding the type I error constraint. For example, in the context of credit cards, the type I error reflects the default rate on credit card payments. Financial institutions can establish their own benchmarks based on their risk management policies and prevailing economic conditions. Over recent decades, the credit card delinquency rate—defined as the percentage of credit card holders who fail to make required payments for at least two consecutive months—has varied between 1.5% and 6.8% in the U.S.<sup>3</sup>. Consequently, a lending institution might aim to control its type I error below a target that incorporates these numbers and its specific operational circumstances.

## C Proofs

### C.1 Proof of Theorem 1

Since the proof is long and complex, we would like to outline the major steps in the proof as follows before moving to the complete proof.

1. Let  $p_{s|y} = \mathbb{P}(S = s \mid Y = y)$  and  $f_{y,s}$  be the density function of  $X$  conditional on

$Y = y$  and  $S = s$ , for all  $s \in \{a, b\}$  and  $y \in \{0, 1\}$ . Moreover, define

$$\begin{aligned}\phi_{c_a, c_b}(X, S) &= \mathbb{I} \left\{ \frac{f_{1,a}(X)}{f_{0,a}(X)} > c_a \frac{p_{a|0}}{p_{a|1}} \right\} \mathbb{I}\{S = a\} \\ &\quad + \mathbb{I} \left\{ \frac{f_{1,b}(X)}{f_{0,b}(X)} > c_b \frac{p_{b|0}}{p_{b|1}} \right\} \mathbb{I}\{S = b\},\end{aligned}$$

for any strictly positive  $c_a, c_b$ . Under mild conditions, the NP oracle classifier (without EO component) whose type I error  $R_0 = \alpha$  can be written as  $\phi_{c_\alpha, c_\alpha}$  by Neyman-Pearson lemma, where  $c_\alpha$  is chosen such that  $R_0(\phi_{c_\alpha, c_\alpha}) = \alpha$ . Then, there are two cases:  $\phi_{c_\alpha, c_\alpha}$  satisfies  $L_1 \leq \varepsilon$ , and  $\phi_{c_\alpha, c_\alpha}$  satisfies  $L_1 > \varepsilon$ . In the first case, the NP oracle classifier is an NP-EO oracle classifier, and thus, we only need to consider the second case. It is also assumed that, without loss of generality, that  $R_1^b(\phi_{c_\alpha, c_\alpha}) - R_1^a(\phi_{c_\alpha, c_\alpha}) > \varepsilon$ .

2. It can be shown that, invoking generalized Neyman-Pearson lemma (Theorem S.3), as long as there exist  $C$  and  $C'$  with  $0 < C' < C$  such that the classifier

$$\begin{aligned}\phi^*(X, S) := \phi_{C, C'}(X, S) &= \mathbb{I} \left\{ \frac{f_{1,a}(X)}{f_{0,a}(X)} > C \frac{p_{a|0}}{p_{a|1}} \right\} \mathbb{I}\{S = a\} \\ &\quad + \mathbb{I} \left\{ \frac{f_{1,b}(X)}{f_{0,b}(X)} > C' \frac{p_{b|0}}{p_{b|1}} \right\} \mathbb{I}\{S = b\}\end{aligned}$$

satisfies  $R_0(\phi^*) = \alpha$  and  $R_1^b(\phi^*) - R_1^a(\phi^*) = \varepsilon$ ,  $\phi^*$  is a solution to the following optimization problem

$$\text{minimize } R_1(\phi),$$

$$\text{subject to } R_0(\phi) \leq \alpha \quad \text{and} \quad R_1^b(\phi) - R_1^a(\phi) \leq \varepsilon.$$

Given  $R_1^b(\phi^*) - R_1^a(\phi^*) = \varepsilon$ ,  $\phi^*$  is also a solution to the same optimization problem over the smaller set of NP-EO classifiers

$$\begin{aligned} & \text{minimize } R_1(\phi), \\ & \text{subject to } R_0(\phi) \leq \alpha \quad \text{and} \quad -\varepsilon \leq R_1^b(\phi) - R_1^a(\phi) \leq \varepsilon. \end{aligned}$$

Thus,  $\phi^*$  is an NP-EO oracle classifier.

3. Note that  $R_0(\phi_{c_a, c_b})$  is decreasing in both  $c_a$  and  $c_b$ . Moreover  $R_1^a(\phi_{c_a, c_b})$  and  $R_1^b(\phi_{c_a, c_b})$  are increasing in  $c_a$  and  $c_b$ , respectively. Under mild assumptions, starting from  $R_1^b(\phi_{c_\alpha, c_\alpha}) - R_1^a(\phi_{c_\alpha, c_\alpha}) > \varepsilon$  and  $R_0(\phi_{c_\alpha, c_\alpha}) = \alpha$ , we show that there exist  $C, C'$  such that  $0 < C' < c_\alpha < C$  and  $R_1^b(\phi_{C, C'}) - R_1^a(\phi_{C, C'}) = \varepsilon$  and  $R_0(\phi_{C, C'}) = \alpha$ . Then,  $\phi_{C, C'}$  is an NP-EO oracle classifier.

Now let us proceed with the detailed proof. First, we state the mathematical foundation for the densities. Let  $\mu = \mu_d \times \mathcal{M}$  be a measure defined on  $\mathbb{R}^d \times \{a, b\}$ , where  $\mu_d$  is Lebesgue measure on  $\mathbb{R}^d$  and  $\mathcal{M}$  is the counting measure on  $\{a, b\}$ . Thus, the random variable  $(X, S) \mid \{Y = 0\}$  and  $(X, S) \mid \{Y = 1\}$  both have densities with respect to  $\mu$ ; denote them by  $f_1$  and  $f_0$  respectively.

Consider the NP oracle (without  $\varepsilon$ -separation constraint). That is, a classifier that minimizes  $R_1$  among all classifiers  $\phi$  such that  $R_0(\phi) \leq \alpha$ . Assume for simplicity that there exists a constant  $c_\alpha$  such that

$$\mathbb{P} \left( \frac{f_1(X, S)}{f_0(X, S)} > c_\alpha \mid Y = 0 \right) = \alpha.$$

By the Neyman-Pearson lemma, the classifier

$$\begin{aligned}\phi_\alpha^{**}(X, S) &= \mathbb{I} \left\{ \frac{f_1(X, S)}{f_0(X, S)} > c_\alpha \right\} \\ &= \sum_{s=a,b} \mathbb{I} \left\{ \frac{f_{1,s}(X)}{f_{0,s}(X)} > c_\alpha \cdot \frac{\mathbb{P}(S=s|Y=0)}{\mathbb{P}(S=s|Y=1)} \right\} \cdot \mathbb{I}\{S=s\},\end{aligned}$$

is the NP oracle classifier. Note that

$$\begin{aligned}\mathbb{P} \left( \frac{f(X | S, Y=1)\mathbb{P}(S | Y=1)}{f(X | S, Y=0)\mathbb{P}(S | Y=0)} > z \mid Y=0 \right) \\ &= \mathbb{P} \left( \frac{f(X | S, Y=1)\mathbb{P}(S | Y=1)}{f(X | S, Y=0)\mathbb{P}(S | Y=0)} > z \mid Y=0, S=a \right) p_{a|0} \\ &\quad + \mathbb{P} \left( \frac{f(X | S, Y=1)\mathbb{P}(S | Y=1)}{f(X | S, Y=0)\mathbb{P}(S | Y=0)} > z \mid Y=0, S=b \right) p_{b|0} \\ &= \left( 1 - F_{0,a} \left( zp_{a|0}p_{a|1}^{-1} \right) \right) p_{a|0} + \left( 1 - F_{0,b} \left( zp_{b|0}p_{b|1}^{-1} \right) \right) p_{b|0}.\end{aligned}$$

Note that  $\lim_{z \rightarrow \infty} F_{0,a}(z) = 1$  and  $F_{0,a}(0) = 0$  by assumption. Similarly,  $F_{0,b}$  has the same property. Then, since both  $F_{0,a}$  and  $F_{0,b}$  are continuous, there exists a  $c_\alpha > 0$  such that the above quantity equals  $\alpha$ . Note that  $\phi_\alpha^{**}$  can be written in the following way.

$$\phi_\alpha^{**}(X, S) = \mathbb{I} \left\{ \frac{f_{1,a}(X)}{f_{0,a}(X)} > c_a^{**} \right\} \mathbb{I}\{S=a\} + \mathbb{I} \left\{ \frac{f_{1,b}(X)}{f_{0,b}(X)} > c_b^{**} \right\} \mathbb{I}\{S=b\},$$

where  $c_a^{**} = c_\alpha p_{0,a} p_{1,a}^{-1}$  and  $c_b^{**} = c_\alpha p_{0,b} p_{1,b}^{-1}$ . Thus,  $\phi_\alpha^{**} = \phi_{c_a^{**}, c_b^{**}}^\#$ .

Now, there are two cases,  $L_1 \left( \phi_{c_a^{**}, c_b^{**}}^\# \right) \leq \varepsilon$  or  $L_1 \left( \phi_{c_a^{**}, c_b^{**}}^\# \right) > \varepsilon$ . For the first case,  $\phi_{c_a^{**}, c_b^{**}}^\#$  minimizes  $R_1$  over  $\{\phi : R_0(\phi) \leq \alpha, L_1(\phi) \leq \varepsilon\}$  since it is the NP oracle classifier and thus  $\phi_{c_a^{**}, c_b^{**}}^\# = \phi_{\alpha, \varepsilon}^*$ .

For the second case, assume without loss of generality,  $R_1^b \left( \phi_{c_a^{**}, c_b^{**}}^\# \right) - R_1^a \left( \phi_{c_a^{**}, c_b^{**}}^\# \right) > \varepsilon$ .

Consider the following optimization problem. For any classifier,

$$\begin{aligned}
& \text{maximize } \mathbb{P}(\phi(X, S) = 1 \mid Y = 1) = \int \phi f(x \mid S = s, Y = 1) \mathbb{P}(S = s \mid Y = 1) d\mu_d, \\
& \text{subject to } R_0(\phi) = \int \phi f(x \mid S = s, Y = 0) \mathbb{P}(S = s \mid Y = 0) d\mu_d = \alpha \\
& R_1^b(\phi) - R_1^a(\phi) \\
& = \int \phi (f_{1,a}(x) \mathbb{I}\{S = a\} - f_{1,b}(x) \mathbb{I}\{S = b\}) d\mu_d = \varepsilon.
\end{aligned} \tag{7}$$

Here, recall that  $\mu_d$  is the Lebesgue measure on  $\mathbb{R}^d$ . By the generalized Neyman-Pearson lemma<sup>4</sup>, if there exist two non-negative numbers  $k_1, k_2$  such that the classifier

$$\begin{aligned}
\phi'(X, S) &= \mathbb{I}\{f_{1,S}(X)p_{S|1} > k_1 f_{0,S}(X)p_{S|0} + k_2 (f_{1,a}(X) \mathbb{I}\{S = a\} - f_{1,b}(X) \mathbb{I}\{S = b\})\} \\
&= \mathbb{I}\left\{\frac{f_{1,a}(X)}{f_{0,a}(X)} > \frac{k_1 p_{a|0}}{p_{a|1} - k_2}\right\} \mathbb{I}\{S = a\} + \mathbb{I}\left\{\frac{f_{1,b}(X)}{f_{0,b}(X)} > \frac{k_1 p_{b|0}}{p_{b|1} + k_2}\right\} \mathbb{I}\{S = b\},
\end{aligned}$$

satisfies  $R_0(\phi') = \alpha$  and  $R_1^b(\phi) - R_1^a(\phi) = \varepsilon$ , it maximizes  $\mathbb{P}(\phi(X, S) = 1 \mid Y = 1)$ , i.e., minimizes  $R_1(\phi)$  over all  $\phi$  such that  $R_0(\phi) \leq \alpha$  and  $R_1^b(\phi) - R_1^a(\phi) \leq \varepsilon$ , and thus validates the assertion in the theorem. Therefore, it suffices to show the existence of  $k_1$  and  $k_2$ . In particular,  $k_1 > 0$  and  $k_2 \in (0, p_{a|1})$ . We claim that there exist two constants  $C > C' > 0$  such that

$$R_0\left(\phi_{C p_{a|0} p_{a|1}^{-1}, C' p_{b|0} p_{b|1}^{-1}}^\#\right) = \alpha, \tag{8}$$

---

<sup>4</sup>Theorem 3.6.1 in Lehmann and Ramano [2005]. It is reproduced as Theorem S.3 in the Appendix for the readers' convenience.

and

$$R_1^b \left( \phi_{Cp_{a|0}p_{a|1}^{-1}, C'p_{b|0}p_{b|1}^{-1}}^\# \right) - R_1^a \left( \phi_{Cp_{a|0}p_{a|1}^{-1}, C'p_{b|0}p_{b|1}^{-1}}^\# \right) = \varepsilon. \quad (9)$$

In view of this, take

$$k_1 = \frac{CC'}{Cp_{b|1} + C'p_{a|1}} \text{ and } k_2 = \frac{C - C'}{Cp_{a|1}^{-1} + C'p_{b|1}^{-1}},$$

and  $\phi'$  satisfies the conditions of optimization problem (7). Moreover, one can see  $k_1 > 0$

and  $k_2 \in (0, p_{a|1})$  since  $C > C' > 0$  and

$$k_2 = \frac{C - C'}{Cp_{a|1}^{-1} + C'p_{b|1}^{-1}} < \frac{C}{Cp_{a|1}^{-1}} = p_{a|1}.$$

Then, generalized Neyman-Pearson lemma validates the assertion. The remaining proof relies on the following two key functions For  $c \in [c_\alpha, \infty)$ ,

$$f(c) = \inf \left\{ z \geq 0 : \left( 1 - F_{0,a}(cp_{a|0}p_{a|1}^{-1}) \right) p_{a|0} + \left( 1 - F_{0,b}(zp_{b|0}p_{b|1}^{-1}) \right) p_{b|0} \leq \alpha \right\}.$$

Conceptually, for a classifier whose  $S = a$  section threshold is  $cp_{a|0}p_{a|1}^{-1}$  and overall type I error is equal to or less than  $\alpha$ ,  $f(c)$  describes its smallest possible  $S = b$  section threshold.

Moreover, define

$$g(c) = \sup \left\{ z \geq 0 : F_{1,b}(zp_{b|0}p_{b|1}^{-1}) - F_{1,a}(cp_{a|0}p_{a|1}^{-1}) = \varepsilon \right\}.$$

on  $[c_\alpha, V)$  where  $V = \sup\{z : F_{1,a}(zp_{b|0}p_{b|1}^{-1}) \leq 1 - \varepsilon\}$ . If a classifier whose  $S = a$

section threshold is  $c$  satisfies the  $\varepsilon$ -separation,  $g(c)$  describes the largest possible  $S = b$  section threshold. To check the domain of  $g$  is indeed well defined, i.e.,  $c_\alpha < V$ , note that by our assumption that  $F_{1,b}(c_\alpha p_{b|0} p_{b|1}^{-1}) - F_{1,a}(c_\alpha p_{a|0} p_{a|0}^{-1}) > \varepsilon$ , one can conclude that  $F_{1,a}(c_\alpha p_{b|0} p_{b|1}^{-1}) < 1 - \varepsilon$  and thus  $c_\alpha < V$  by continuity of  $F_{1,a}$ . Here, we make several remarks that are useful in the following proofs

- $f$  is non-increasing whereas  $g$  is positive and non-decreasing;
- By the definition of  $c_\alpha$ ,  $0 < g(c_\alpha) < c_\alpha$  and  $f(c_\alpha) \leq c_\alpha$ ;
- By continuity of  $F_{y,s}$  for every  $y$  and  $s$ , if  $f(c) > 0$ ,

$$\left(1 - F_{0,a}(c p_{a|0} p_{a|1}^{-1})\right) p_{a|0} + \left(1 - F_{0,b}(f(c) p_{b|0} p_{b|1}^{-1})\right) p_{b|0} = \alpha,$$

and

$$F_{1,b}(g(c) p_{b|0} p_{b|1}^{-1}) - F_{1,a}(c p_{a|0} p_{a|0}^{-1}) = \varepsilon.$$

Then, it remains to discuss several scenarios. If  $f(c_\alpha) \leq g(c_\alpha)$ , then the existence of  $C > C' > 0$  is given by Lemma S.1. The scenario where  $f(c_\alpha) > g(c_\alpha)$  is more involved. Let  $\mathcal{A}^- = \{c \in [c_\alpha, V) : g(c) < f(c)\}$  and  $\mathcal{A}^+ = \{c \in [c_\alpha, V) : g(c) \geq f(c)\}$ . Furthermore, denote  $A = \sup \mathcal{A}^-$ . Depending on if  $A < V$  or  $A = V$ , this scenario is further divided into two cases. For  $A < V$ , the proof is finished by Lemma S.2. Otherwise, the proof is done by Lemma S.3.

## C.2 Proof of Proposition 1

Let  $p_1, p_2 \in (0, 1)$  be two distinct numbers. Moreover, define  $(X_{p_1}, S_{p_1}, Y_{p_1})$  and  $(X_{p_2}, S_{p_2}, Y_{p_2})$  be random triplets with the same distributions except  $\mathbb{P}(Y_{p_1} = 0) = p_1$  and  $\mathbb{P}(Y_{p_2} = 0) = p_2$ , respectively. For any  $p \in \{p_1, p_2\}$  and arbitrary classifier  $\phi$ , we denote  $R_q^s(\phi \mid p)$  to be the  $R_q^s$  of  $\phi$  based on the random variable  $(X_p, S_p, Y_p)$  for any  $s \in \{a, b\}$  and  $q \in \{0, 1\}$ . Similarly,  $R_0(\phi \mid p)$  and  $R_1(\phi \mid p)$  are the type I error and type II errors of  $\phi$  based on  $(X_p, S_p, Y_p)$ .

Note that by assumption,  $X_{p_1} \mid (S_{p_1} = s, Y_{p_1} = s)$  actually has the same distribution as  $X_{p_2} \mid (S_{p_2} = s, Y_{p_2} = s)$  for each  $s \in \{a, b\}, q \in \{0, 1\}$ . Then, for every  $z \in [0, \infty)$ ,

$$\mathbb{P} \left( \frac{f_{1,s}(X_{p_1})}{f_{0,s}(X_{p_1})} \leq z \mid Y_{p_1} = q, S_{p_1} = s \right) = \mathbb{P} \left( \frac{f_{1,s}(X_{p_2})}{f_{0,s}(X_{p_2})} \leq z \mid Y_{p_2} = q, S_{p_2} = s \right),$$

for each  $s \in \{a, b\}, q \in \{0, 1\}$ . This further implies that, given a classifier  $\phi_{c_a, c_b}^\#$  of the form in equation (5) for arbitrary constants  $c_a$  and  $c_b$ ,  $R_q^s(\phi_{c_a, c_b}^\# \mid p_1) = R_q^s(\phi_{c_a, c_b}^\# \mid p_2)$ . Thus,

$$\begin{aligned} R_0(\phi_{c_a, c_b}^\# \mid p_1) &= R_0^a(\phi_{c_a, c_b}^\# \mid p_1)p_{a|0} + R_0^b(\phi_{c_a, c_b}^\# \mid p_1)p_{b|0} \\ &= R_0^a(\phi_{c_a, c_b}^\# \mid p_2)p_{a|0} + R_0^b(\phi_{c_a, c_b}^\# \mid p_2)p_{b|0} \\ &= R_0(\phi_{c_a, c_b}^\# \mid p_2). \end{aligned}$$

Moreover,

$$R_1^a(\phi_{c_a, c_b}^\# \mid p_1) - R_1^b(\phi_{c_a, c_b}^\# \mid p_1) = R_1^a(\phi_{c_a, c_b}^\# \mid p_2) - R_1^b(\phi_{c_a, c_b}^\# \mid p_2).$$

Denote  $\phi_{p_1}^\#$  and  $\phi_{p_2}^\#$  to be NP-EO oracle classifiers for  $(X_{p_1}, S_{p_1}, Y_{p_1})$  and  $(X_{p_2}, S_{p_2}, Y_{p_2})$ ,

respectively. Since  $\phi_{p_1}^\#$  is an NP-EO oracle classifier for  $(X_{p_1}, S_{p_1}, Y_{p_1})$ , it is also an NP-EO classifier for  $(X_{p_2}, S_{p_2}, Y_{p_2})$ . Similarly,  $\phi_{p_2}^\#$  is also an NP-EO classifier for  $(X_{p_1}, S_{p_1}, Y_{p_1})$ .

To this end, it suffices to verify the  $\phi_{p_1}^\#$  achieves the minimum  $R_1$  for  $(X_{p_2}, S_{p_2}, Y_{p_2})$  among all NP-EO classifier. Indeed, since  $\phi_{p_1}^\#$  is also of the form in equation (5),

$$\begin{aligned} R_1(\phi_{p_1}^\# \mid p_1) &= R_1^a(\phi_{p_1}^\# \mid p_1)p_{a|1} + R_1^b(\phi_{p_1}^\# \mid p_1)p_{b|1} \\ &= R_0^a(\phi_{p_1}^\# \mid p_2)p_{a|1} + R_0^b(\phi_{p_1}^\# \mid p_2)p_{b|1} \\ &= R_1(\phi_{p_1}^\# \mid p_2). \end{aligned}$$

Similarly,  $R_1(\phi_{p_2}^\# \mid p_1) = R_1(\phi_{p_2}^\# \mid p_2)$ . If  $R_1(\phi_{p_2}^\# \mid p_2) < R_1(\phi_{p_1}^\# \mid p_2)$ , one can conclude that  $R_1(\phi_{p_2}^\# \mid p_1) < R_1(\phi_{p_1}^\# \mid p_1)$ , violating the fact that  $\phi_{p_1}^\#$  is an NP-EO oracle classifier. Therefore, one can conclude  $R_1(\phi_{p_2}^\# \mid p_2) \geq R_1(\phi_{p_1}^\# \mid p_2)$ , and since  $\phi_{p_2}^\#$  is also an NP-EO oracle classifier,  $R_1(\phi_{p_2}^\# \mid p_2) = R_1(\phi_{p_1}^\# \mid p_2)$ . Therefore,  $\phi_{p_1}^\#$  achieves the minimum  $R_1$  for  $(X_{p_2}, S_{p_2}, Y_{p_2})$  among all NP-EO classifiers.

### C.3 Proof of Theorem 2

The first assertion in this theorem is simple. By Theorem S.1,

$$\mathbb{P} \left( \mathbb{P}_{X^{0,a}} \left( T^a(X^{0,a}) > t_{k_*^{0,a}}^{0,a} \right) > \alpha \right) \leq \delta/2,$$

and

$$\mathbb{P} \left( \mathbb{P}_{X^{0,b}} \left( T^b(X^{0,b}) > t_{k_*^{0,b}}^{0,b} \right) > \alpha \right) \leq \delta/2.$$

Given  $R_0(\widehat{\phi}^*)$  can be written as

$$\mathbb{P}_{X^{0,a}} \left( T^a(X^{0,a}) > t_{k_a^*}^{1,a} \right) \mathbb{P}(S = a \mid Y = 0) + \mathbb{P}_{X^{0,b}} \left( T^b(X^{0,b}) > t_{k_b^*}^{1,b} \right) \mathbb{P}(S = b \mid Y = 0),$$

along with the fact that  $t_{k_a^*}^{1,a} \geq t_{k_*^{0,a}}^{0,a}$  and  $t_{k_b^*}^{1,b} \geq t_{k_*^{0,b}}^{0,b}$ , one can conclude that

$$\begin{aligned} \mathbb{P} \left( R_0(\widehat{\phi}^*) > \alpha \right) &\leq \mathbb{P} \left( \mathbb{P}_{X^{0,a}} \left( T^a(X^{0,a}) > t_{k_*^{0,a}}^{0,a} \right) \mathbb{P}(S = a \mid Y = 0) > \alpha \mathbb{P}(S = a \mid Y = 0) \right) \\ &\quad + \mathbb{P} \left( \mathbb{P}_{X^{0,b}} \left( T^b(X^{0,b}) > t_{k_*^{0,b}}^{0,b} \right) \mathbb{P}(S = b \mid Y = 0) > \alpha \mathbb{P}(S = b \mid Y = 0) \right) \\ &\leq \delta. \end{aligned}$$

Next, we proceed to the second assertion. Before presenting the proof, we remark that as long as  $l_a, l_b, n_a$  and  $n_b$  are fixed, Algorithm 3 is a deterministic procedure. That is,  $k_a^* = k_a^*(l_a, l_b, n_a, n_b)$  is a non-random quantity and neither is  $k_b^*$ .

Now, let us focus on the proof. We denote the classifier given by Algorithm 1 is

$$\widehat{\phi}^*(X, S) = \mathbb{I}\{T^a(X) > t_{k_a^*}^{1,a}\} \mathbb{I}\{S = a\} + \mathbb{I}\{T^b(X) > t_{k_b^*}^{1,b}\} \mathbb{I}\{S = b\}.$$

Let  $\xi_j^a = \mathbb{I}\{t_j^{1,a} \leq t_{(k_*^{0,a})}^{0,a}\}$  for every  $t_j^{1,a} \in \mathcal{T}^{1,a}$  and  $\xi_i^b = \mathbb{I}\{t_i^{1,b} \leq t_{(k_*^{0,b})}^{0,b}\}$  for every  $t_i^{1,b} \in \mathcal{T}^{1,b}$ .

Note that

$$\mathbb{P} \left( |R_1^a - R_1^b| > \varepsilon \right) = \mathbb{E}_{\mathcal{S}_{\text{train}}} \left[ \mathbb{P}_{\text{left-out}} \left( |R_1^a - R_1^b| > \varepsilon \right) \right].$$

The probability  $\mathbb{P}_{\text{left-out}}$  is taken with respect to the randomness of all  $\mathcal{S}_{\text{left-out}}^{y,s}$ . If this quantity can be shown to be at most  $\gamma$ , then  $\mathbb{P} \left( |R_1^a - R_1^b| > \varepsilon \right) \leq \gamma$ . Thus, till the end of

the proof, we will only consider the randomness in  $\mathbb{P}_{\text{left-out}}$  and take  $T^a$  and  $T^b$  to be fixed.

Next, note that

$$\mathbb{P}_{\text{left-out}}(|R_1^a - R_1^b| > \varepsilon) = \mathbb{E}_\xi \mathbb{P}_{\text{left-out}}(|R_1^a - R_1^b| > \varepsilon \mid \xi_1^a, \dots, \xi_{n_a}^a, \xi_1^b, \dots, \xi_{n_b}^b)$$

where  $\mathbb{E}_\xi$  is the expectation taken with respect to  $\xi_1^a, \dots, \xi_{n_a}^a, \xi_1^b, \dots, \xi_{n_b}^b$ . Moreover, denote

$\xi^a = (\xi_1^a, \xi_2^a, \dots, \xi_{n_a}^a)$  and  $\xi^b = (\xi_1^b, \xi_2^b, \dots, \xi_{n_b}^b)$ . To this end, we will show  $\mathbb{P}_{\text{left-out}}(|R_1^a - R_1^b| > \varepsilon \mid \xi^a, \xi^b)$

is bounded by approximately  $\gamma$  with high probability. Consider the quantity

$$R_1^a = R_1^a(\widehat{\phi}^*) = \mathbb{P}_{\text{left-out}}\left(T^a(X^{1,a}) \leq t_{(k_a^*)}^{1,a}\right).$$

We remark that conditional on  $\mathcal{S}_{\text{train}}$ ,  $R_1^a$  is solely determined by  $\mathcal{S}_{\text{left-out}}^{0,a}$  and  $\mathcal{S}_{\text{left-out}}^{1,a}$ . Thus,

$R_1^a$  is independent of  $\xi^b$ . Furthermore, conditional on  $\xi^a$ ,  $k_a^*$  is fixed. Thus, denote  $k_a^* = k_a$ ,

for any  $s \in \mathbb{R}$  the conditional distribution function of  $R_1^a$  can be written as

$$\mathbb{P}_{\text{left-out}}[R_1^a \leq s \mid \xi^a, \xi^b] = \mathbb{P}_{\text{left-out}}[R_1^a \leq s \mid \xi^a] = \mathbb{E}_{t_{k_*}^{0,a}} \left[ \mathbb{P}_{\text{left-out}}\left(R_1^a \leq s \mid \xi^a, t_{k_*}^{0,a}\right) \mid \xi^a \right].$$

Define  $G_a = \mathbb{P}_{\text{left-out}}\left(t^{1,a} \leq t_{(k_*^{0,a})}^{0,a} \mid t_{(k_*^{0,a})}^{0,a}\right)$  where  $t^{1,a}$  is another iid copy of  $t_1^{1,a}, \dots, t_{n_a}^{1,a}$ ,

then conditional on  $\xi^a$  and  $t_{k_*}^{0,a}$ ,  $R_1^a$  is equal to distribution to  $G_a + (1 - G_a) B_a$  where  $B_a$  is

beta distributed with parameters  $k_a - l_a$  and  $n_a^1 - k_a + 1$  by Lemma S.4. Here,  $l_a = \sum_{j=1}^{n_a} \xi_j^a$ .

Then, since

$$\begin{aligned} \mathbb{P}_{\text{left-out}}[R_1^a \leq s \mid \xi^a] &= \mathbb{E}_{t_{k_*}^{0,a}} \left[ \mathbb{P}_{\text{left-out}}\left(R_1^a \leq s \mid \xi^a, t_{k_*}^{0,a}\right) \mid \xi^a \right] \\ &= \mathbb{E}_{t_{k_*}^{0,a}} [\mathbb{P}_{B_a}(G_a + (1 - G_a) B_a \leq s) \mid \xi^a] \end{aligned}$$

$$\begin{aligned}
&= \mathbb{E}_{B_a} \mathbb{P}_{t_{k_*^{0,a}}^{0,a}} (G_a + (1 - G_a) B_a \leq s \mid \xi^a) \\
&= \mathbb{E}_{B_a} \mathbb{P}_{F_a} (F_a + (1 - F_a) B_a \leq s),
\end{aligned}$$

where  $F_a$  is a random variable such that  $\mathbb{P}_{F_a}(F_a \leq t) = \mathbb{P}_{t_{k_*^{0,a}}^{0,a}}(G_a \leq t \mid \xi^a)$  for any constant  $t$ . Here, we use the fact  $G_a$  is constant conditional on  $t_{k_*^{0,a}}^{0,a}$  for the second equality and  $B_a$  is independent of  $t_{k_*^{0,a}}^{0,a}$  and  $\xi^a$  for the third equality. Therefore, the distribution of  $R_1^a \mid \xi^a$  is equal to  $F_a + (1 - F_a)B_a$ . Similarly,  $R_1^b \mid \xi^b$  has the same distribution as  $F_b + (1 - F_b)B_b$  where  $F_b$  and  $B_b$  are defined analogously.

Let  $V_a = F_a + (1 - W_a)B_a$  and  $V_b = F_b + (1 - W_b)B_b$ . Given that  $R_1^a$  and  $R_1^b$  are independent,

$$\mathbb{P}_{\text{left-out}}(|R_1^a - R_1^b| > \varepsilon \mid \xi^a, \xi^b) = \mathbb{P}_{\text{left-out}}(|V_a - V_b| > \varepsilon \mid \xi^a, \xi^b).$$

It remains to show that the distributions of  $F_a$  and  $F_b$  are close to Gaussian distributions described in Algorithm 3. This is true by Bernstein-von Mises theorem. In detail, it is not hard to realize that  $\mathbb{P}_{F_a}(F_a \leq t) = \mathbb{P}_{t_{k_*^{0,a}}^{0,a}}(G_a \leq t \mid \xi^a)$  is exactly the posterior distribution of  $G_a$  given  $\xi^a$ . One can show that  $\xi^a$  is exactly the vector of independent Bernoulli random variables with a success rate  $G_a$ . Moreover, for fixed  $t_{k_*^{0,a}}^{0,a}$ ,  $l_a/n_a^1$  is the maximum likelihood estimator of  $G_a$  by the definition of  $l_a$  in display (9). Then, Bernstein-von Mises theorem states that

$$\left\| \mathbb{P}_{F_a}(F_a \in \cdot \mid \xi^a, \xi^b) - \mathcal{N}\left(\frac{l_a}{n_a^1}, \frac{G_a^*(1 - G_a^*)}{n_a^1}\right) \right\|_{TV} \rightarrow 0,$$

in probability, where  $G_a^*$  is the true success probability of the Bernoulli distribution from

which the Bernoulli trials  $\xi^a$  are generated. Furthermore,

$$\left\| \mathcal{N} \left( \frac{l_a}{n_a^1}, \frac{G_a^*(1 - G_a^*)}{n_a^1} \right) - \mathcal{N} \left( \frac{l_a}{n_a^1}, \frac{(l_a/n_a^1)(1 - l_a/n_a^1)}{n_a^1} \right) \right\|_{TV} \rightarrow 0,$$

in probability as  $l_a/n_a^1$  converges to  $G_a^*$  in probability. Therefore,

$$\left\| \mathbb{P}_{F_a} (F_a \in \cdot \mid \xi^a, \xi^b) - \mathcal{N} \left( \frac{l_a}{n_a}, \frac{(l_a/n_a^1)(1 - l_a/n_a^1)}{n_a^1} \right) \right\|_{TV} \rightarrow 0,$$

in probability. That is, for any  $\varepsilon', \gamma'$  and sufficiently large  $n_a$ ,

$$\sup_B \left| \mathbb{P}_{F_a} (F_a \in B \mid \xi^a, \xi^b) - \mathbb{P}_{Z_a} (Z_a \in B) \right| \leq \varepsilon',$$

with probability at least  $1 - \gamma'/2$  where  $Z_a \sim \mathcal{N}(l_a/n_a, \frac{(l_a/n_a)(1-l_a/n_a)}{n_a})$ . Here, the supremum is taken with respect to all measurable sets. Similarly, for sufficiently large  $n_b$

$$\sup_B \left| \mathbb{P}_{F_b} (F_b \in B \mid \xi^a, \xi^b) - \mathbb{P}_{Z_b} (Z_b \in B) \right| \leq \varepsilon',$$

with probability at least  $1 - \gamma'/2$ . Therefore, denoting  $V'_a = Z_a + (1 - Z_a)B_a$  and  $V'_b = Z_b + (1 - Z_b)B_b$ , with probability at least  $1 - \gamma'$ ,

$$\begin{aligned} \mathbb{P}_{\text{left-out}} (|R_1^a - R_1^b| > \varepsilon \mid \xi^a, \xi^b) &= \mathbb{E}_{W_a} \mathbb{E}_{W_b} \mathbb{E}_{B_a} \mathbb{E}_{B_b} \mathbb{I}\{|V_a - V_b| > \varepsilon\} \\ &\leq \mathbb{E}_{Z_a} \mathbb{E}_{Z_b} \mathbb{E}_{B_a} \mathbb{E}_{B_b} \mathbb{I}\{|V'_a - V'_b| > \varepsilon\} + \varepsilon' + (\varepsilon')^2. \end{aligned}$$

The expectation term on the right-hand side of the inequality is  $\gamma$  by design of Algorithm

1. Therefore,

$$\mathbb{E}_\xi \mathbb{P}_{\text{left-out}} \left( |R_1^a - R_1^b| > \varepsilon \mid \xi^a, \xi^b \right) \leq \gamma + \varepsilon' + (\varepsilon')^2 + \gamma'.$$

Let  $\xi(n_a^1, n_b^1) = \varepsilon' + (\varepsilon')^2 + \gamma'$ . Then,  $\xi(n_a^1, n_b^1)$  is a function of  $n_a^1$  and  $n_b^1$  that converges to 0 as  $n_a^1$  and  $n_b^1$  go to infinity, and the proof is finished.

## C.4 Proof of Theorem 3

We start with the proof of the NP part. By NP umbrella algorithm (S.1), with probability at least  $1 - \delta$ ,  $R_0(\widehat{\phi}_*) \leq \alpha$ , where  $\widehat{\phi}_*$  is defined in (1). Next, let  $\widehat{R}_0(\phi)$  be the empirical type I error of a classifier  $\phi$ . It is not hard to see that

$$\widehat{R}_0(\widehat{\phi}_*) = \frac{1}{n_a^0 + n_b^0} \left( \sum_{i=1}^{n_a^0} \mathbb{I}\{t_i^{0,a} > t_{(k_*)}^0\} + \sum_{j=1}^{n_b^0} \mathbb{I}\{t_j^{0,b} > t_{(k_*)}^0\} \right).$$

Next, for any  $c_a, c_b \in \mathbb{R}$ , define

$$\widehat{\phi}_{c_a, c_b}(X, S) = \mathbb{I}\{T^a(X) > c_a\} \mathbb{I}\{S = a\} + \mathbb{I}\{T^b(X) > c_b\} \mathbb{I}\{S = b\}.$$

By the definition of  $k_a^0$  and  $k_b^0$  in (2), if  $t_{(k_a^0)}^{0,a}$  and  $t_{(k_b^0)}^{0,b}$  are chosen as the thresholds,

$$\begin{aligned} \widehat{R}_0 \left( \widehat{\phi}_{t_{(k_a^0)}^{0,a}, t_{(k_b^0)}^{0,b}} \right) &= \frac{1}{n_a^0 + n_b^0} \left( \sum_{i=1}^{n_a^0} \mathbb{I}\{t_i^{0,a} > t_{(k_a^0)}^{0,a}\} + \sum_{j=1}^{n_b^0} \mathbb{I}\{t_j^{0,b} > t_{(k_b^0)}^{0,b}\} \right) \\ &= \frac{1}{n_a^0 + n_b^0} \left( \sum_{i=1}^{n_a^0} \mathbb{I}\{t_i^{0,a} > t_{(k_*)}^0\} + \sum_{j=1}^{n_b^0} \mathbb{I}\{t_j^{0,b} > t_{(k_*)}^0\} \right) = \widehat{R}_0(\widehat{\phi}_*). \end{aligned}$$

Then, for any  $k_a, k_b$  such that  $k_a + k_b = k_a^0 + k_b^0$ ,  $\widehat{R}_0 \left( \widehat{\phi}_{t_{(k_a^0)}^{0,a}, t_{(k_b^0)}^{0,b}} \right) = \widehat{R}_0 \left( \widehat{\phi}_{t_{(k_a)}^{0,a}, t_{(k_b)}^{0,b}} \right) = \widehat{R}_0(\widehat{\phi}_*)$ . Then, for any  $c$ ,

$$\begin{aligned} & \left| R_0 \left( \widehat{\phi}_{t_{(k_a^0)}^{0,a}, t_{(k_b^0)}^{0,b}} \right) - R_0(\widehat{\phi}_*) \right| \\ & \leq \left| R_0 \left( \widehat{\phi}_{t_{(k_a^0)}^{0,a}, t_{(k_b^0)}^{0,b}} \right) - \widehat{R}_0 \left( \widehat{\phi}_{t_{(k_a^0)}^{0,a}, t_{(k_b^0)}^{0,b}} \right) \right| + \left| R_0(\widehat{\phi}_*) - \widehat{R}_0(\widehat{\phi}_*) \right|. \end{aligned}$$

Next, it suffices to bound the two quantities on the right-hand side by  $\eta/2$  respectively.

Note that

$$\begin{aligned} & \left| R_0(\widehat{\phi}_*) - \widehat{R}_0(\widehat{\phi}_*) \right| \\ & \leq \left| \frac{1}{n^0} \left( \sum_{i=1}^{n_a^0} \mathbb{I}\{t_i^{0,a} > t_{(k_*)^0}^0\} + \sum_{j=1}^{n_b^0} \mathbb{I}\{t_j^{0,b} > t_{(k_*)^0}^0\} \right) - \mathbb{P}(T(X, S) > t_{(k_*)^0}^0 \mid Y = 0) \right| \leq \eta/2, \end{aligned}$$

with probability at least  $1 - 2 \exp(-\frac{1}{2}n^0\eta^2)$  by the Dvoretzky-Kiefer-Wolfowitz inequality.

For the concentration of  $\widehat{R}_0 \left( \widehat{\phi}_{t_{(k_a^0)}^{0,a}, t_{(k_b^0)}^{0,b}} \right)$ , we first consider the concentration of  $n_a^0$  and  $n_b^0$ . Define  $\mathcal{A}_\eta = \left\{ \left| \frac{n_a^0}{n^0} - p_{a|0} \right| \leq \frac{\eta}{8} \right\}$ . Hoeffding's inequality implies  $\mathbb{P}(\mathcal{A}_\eta^c) \leq 2 \exp(-\frac{1}{32}n^0\eta^2)$ .

On the event  $\mathcal{A}_\eta$ , note that

$$\begin{aligned} & R_0 \left( \widehat{\phi}_{t_{(k_a^0)}^{0,a}, t_{(k_b^0)}^{0,b}} \right) - \widehat{R}_0 \left( \widehat{\phi}_{t_{(k_a^0)}^{0,a}, t_{(k_b^0)}^{0,b}} \right) \\ & \leq \left( \frac{1}{n_a^0} \sum_{i=1}^{n_a^0} \mathbb{I}\{t_i^{0,a} > t_{(k_a^0)}^{0,a}\} \right) \left( \frac{n_a^0}{n_a^0 + n_b^0} \right) - R_0^a \left( \widehat{\phi}_{t_{(k_a^0)}^{0,a}, t_{(k_b^0)}^{0,b}} \right) p_{a|0} \\ & \quad + \left( \frac{1}{n_b^0} \sum_{i=1}^{n_b^0} \mathbb{I}\{t_i^{0,b} > t_{(k_b^0)}^{0,b}\} \right) \left( \frac{n_b^0}{n_a^0 + n_b^0} \right) - R_0^b \left( \widehat{\phi}_{t_{(k_a^0)}^{0,a}, t_{(k_b^0)}^{0,b}} \right) p_{b|0}. \end{aligned}$$

Since the  $\{S = a\}$  and  $\{S = b\}$  parts are symmetric, we will only focus on the  $\{S = a\}$  part. Note that

$$\begin{aligned} & \left| \left( \frac{1}{n_a^0} \sum_{i=1}^{n_a^0} \mathbb{I}\{t_i^{0,a} > t_{(k_a^0)}^{0,a}\} \right) \left( \frac{n_a^0}{n_a^0 + n_b^0} \right) - R_0^a \left( \hat{\phi}_{t_{(k_a^0)}^{0,a}, t_{(k_b^0)}^{0,b}} \right) p_{a|0} \right| \\ & \leq \left| \frac{1}{n_a^0} \sum_{i=1}^{n_a^0} \mathbb{I}\{t_i^{0,a} > t_{(k_a^0)}^{0,a}\} - R_0^a \left( \hat{\phi}_{t_{(k_a^0)}^{0,a}, t_{(k_b^0)}^{0,b}} \right) \right| + \left| \frac{n_a^0}{n_a^0 + n_b^0} - p_{a|0} \right|. \end{aligned}$$

On  $\mathcal{A}_\eta$ , the second term on the right-hand side of this inequality is at most  $\eta/8$ . It suffices to bound the first term. Note that  $\mathcal{A}_\eta$  is equivalent to  $n^0(p_{a|0} - \eta/8) \leq n_a^0 \leq n^0(p_{a|0} + \eta/8)$ . Thus, on this event, the first term is bounded by  $\eta/8$  with probability at least  $1 - 2 \exp(-\frac{1}{32}n^0(p_{a|0} - \eta/8)\eta^2)$  by Lemma S.9. Apply the same procedure to  $\{S = b\}$  part, one can have similar results. Therefore,

$$\begin{aligned} & \mathbb{P} \left( \sup_{\substack{t_{(k_a^0)}^{0,a}, t_{(k_b^0)}^{0,b}}} \left| R_0 \left( \hat{\phi}_{t_{(k_a^0)}^{0,a}, t_{(k_b^0)}^{0,b}} \right) - \hat{R}_0 \left( \hat{\phi}_{t_{(k_a^0)}^{0,a}, t_{(k_b^0)}^{0,b}} \right) \right| > \frac{\eta}{2} \right) \\ & \leq 2e^{-\frac{1}{32}n^0(p_{a|0} - \eta/8)\eta^2} + 2e^{-\frac{1}{32}n^0(p_{b|0} - \eta/8)\eta^2} + 2e^{-\frac{1}{32}n^0\eta^2}, \end{aligned}$$

and thus

$$\begin{aligned} & \mathbb{P} \left( \sup_{\substack{t_{(k_a^0)}^{0,a}, t_{(k_b^0)}^{0,b}, t_{(k_*)^0}^{0,*}}} \left| R_0 \left( \hat{\phi}_{t_{(k_a^0)}^{0,a}, t_{(k_b^0)}^{0,b}} \right) - R_0(\hat{\phi}_*) \right| > \eta \right) \\ & \leq 2e^{-\frac{1}{32}n^0(p_{a|0} - \eta/8)\eta^2} + 2e^{-\frac{1}{32}n^0(p_{b|0} - \eta/8)\eta^2} + 2e^{-\frac{1}{32}n^0\eta^2} + 2e^{-\frac{1}{2}n^0\eta^2}. \end{aligned}$$

The proof of the second assertion is similar to the proof of Theorem 2. Let us set

$R_1^a := R_1^a(\widehat{\phi}^{**})$  and recall that

$$l_a(i) = \sum_{j=1}^{n_a^1} \mathbb{I} \left\{ t_j^{1,a} \leq t_{(i)}^{0,a} \right\},$$

for  $i \in [n_a^0]$ . One modification we need is to show

$$R_1^a \mid \{l_a(1), l_a(2), \dots, l_a(n_a^0), t_{(1)}^{0,a}, \dots, t_{(n_a^0)}^{0,a}\} \stackrel{d}{=} \begin{cases} B_{k, l_a(1)-k+1} L_1^a, & k \leq l_a(1), \\ L_p^a + (L_{p+1}^a - L_p^a) B_{k-l_a(p), l_a(p+1)-k+1}, & l_a(p) < k \leq l_a(p+1), p \in [n_a^0 - 1], \\ L_{n_a^0}^a + (1 - L_{n_a^0}^a) B_{k-l_a(n_a^0), n_a^1-k+1}, & k > l_a(n_a^0), \end{cases} \quad (10)$$

where  $L_j^a = \mathbb{P}_{\text{left-out}} \left( t_j^{1,a} \leq t_{(j)}^{0,a} \mid t_{(j)}^{0,a} \right)$  for  $j \in [n_a^0]$  and  $t^{1,a}$  is another iid copy of  $t_1^{1,a}, \dots, t_{n_a^1}^{1,a}$ .

However, this is true by Lemma S.8. After this point is validated, one can mimic the proof of Theorem 2 and invoke the Bernstein-von Mises theorem to the multinomial posterior distribution of

$$\left[ L_1^a, L_2^a - L_1^a, L_3^a - L_2^a, \dots, L_{n_a^0}^a - L_{n_a^0-1}^a, n_a^1 - L_{n_a^0}^a \right]^\top$$

given  $\{l_a(1), l_a(2), \dots, l_a(n_a^0)\}$ .

Another modification is that we need to make sure  $n_a^1$  and  $n_b^1$  diverge if  $n^1$  goes to infinity. However, since  $p_{a|1}$  and  $p_{b|1}$  are strictly positive,  $|n_a^1/n^1 - p_{a|1}|$  converges to 0 in probability. This implies  $n_a^1$  diverges with probability converging to 1. Similarly,  $n_b^1$  diverges with probability converging to 1. Then, the remainder of this proof follows the proof of Theorem 2.

## C.5 Lemmas

**Lemma S.1.** *If  $f(c_\alpha) \leq g(c_\alpha)$ , there exist  $C > C' > 0$  that satisfy equations (8) and (9).*

*Proof.* By the definition of  $c_\alpha$ ,

$$\left(1 - F_{0,a}(c_\alpha p_{a|0} p_{a|1}^{-1})\right) p_{a|0} + \left(1 - F_{0,b}(c_\alpha p_{b|0} p_{b|1}^{-1})\right) p_{b|0} = \alpha.$$

Moreover,

$$\left(1 - F_{0,a}(c_\alpha p_{a|0} p_{a|1}^{-1})\right) p_{a|0} + \left(1 - F_{0,b}(f(c_\alpha) p_{b|0} p_{b|1}^{-1})\right) p_{b|0} = \alpha,$$

Since  $f(c_\alpha) \leq g(c_\alpha) < c_\alpha$ , we have

$$\left(1 - F_{0,a}(c_\alpha p_{a|0} p_{a|1}^{-1})\right) p_{a|0} + \left(1 - F_{0,b}(g(c_\alpha) p_{b|0} p_{b|1}^{-1})\right) p_{b|0} = \alpha,$$

by monotonicity of  $F_{0,a}$ . Thus, letting  $C = c_\alpha$  and  $C' = g(c_\alpha)$  yields the desired result.  $\square$

**Lemma S.2.** *If  $f(c_\alpha) > g(c_\alpha)$  and  $A < V$ , there exist  $C > C' > 0$  that satisfy equation 8 and 9.*

*Proof.* By monotonicity of  $f$  and  $g$ , for any  $c \in [c_\alpha, V)$ , one can conclude  $c \in \mathcal{A}^+$  if  $c \in (A, V)$  and  $c \in \mathcal{A}^-$  if  $c \in [c_\alpha, A)$ . Then, we claim that  $A \in \mathcal{A}^+$  since if  $A \in \mathcal{A}^-$ , there exists an  $a \in (g(A), f(A))$ , and, for a sufficiently small positive number  $\delta$ , by continuity of  $F_{0,a}$  and  $F_{1,a}$ , we have

$$\left(1 - F_{0,a}((A + \delta) p_{a|0} p_{a|1}^{-1})\right) p_{a|0} + \left(1 - F_{0,b}(a p_{b|0} p_{b|1}^{-1})\right) p_{b|0} > \alpha,$$

and

$$F_{1,b} \left( ap_{b|0} p_{b|1}^{-1} \right) - F_{1,a} \left( (A + \delta) p_{a|0} p_{a|0}^{-1} \right) < \varepsilon.$$

Thus,  $f(A + \delta) > a > g(A + \delta)$  and  $A + \delta \in \mathcal{A}^-$ , contradicting the fact that  $A + \delta \in \mathcal{A}^+$ .

Furthermore, since  $f(c_\alpha) > g(c_\alpha)$ , replacing  $A$  with  $c_\alpha$  in all previous argument yields the conclusion that  $A > c_\alpha$ .

Now denote  $F = \lim_{c \rightarrow A^-} f(c)$  and  $G = \lim_{c \rightarrow A^-} g(c)$ , whose existence is guaranteed by  $f$  and  $g$  being monotone and bounded by  $f(c) > 0$  and  $g(c) < f(c) \leq f(c_\alpha) \leq c_\alpha$ . Furthermore, we have  $G \geq g(c_\alpha) > 0$  by monotonicity of  $g$  and  $F \geq G$  as  $f > g$  on  $\mathcal{A}^-$ . Then, by continuity of  $F_{0,a}$  and  $F_{0,b}$ ,

$$\begin{aligned} & \left( 1 - F_{0,a}(Ap_{a|0}p_{a|1}^{-1}) \right) p_{a|0} + \left( 1 - F_{0,b}(Fp_{b|0}p_{b|1}^{-1}) \right) p_{b|0} \\ &= \left( 1 - F_{0,a}(Ap_{a|0}p_{a|1}^{-1}) \right) p_{a|0} + \lim_{c \rightarrow A^-} \left( 1 - F_{0,b}(f(c)p_{b|0}p_{b|1}^{-1}) \right) p_{b|0} \\ &= \left( 1 - F_{0,a}(Ap_{a|0}p_{a|1}^{-1}) \right) p_{a|0} + \lim_{c \rightarrow A^-} \left[ \alpha - \left( 1 - F_{0,a}(cp_{a|0}p_{a|1}^{-1}) \right) p_{a|0} \right] = \alpha. \quad (11) \end{aligned}$$

Similarly, we have

$$\begin{aligned} F_{1,b} \left( Gp_{b|0}p_{b|1}^{-1} \right) - F_{1,a} \left( Ap_{a|0}p_{a|0}^{-1} \right) &= \lim_{c \rightarrow A^-} F_{1,b} \left( g(c)p_{b|0}p_{b|1}^{-1} \right) - F_{1,a} \left( Ap_{a|0}p_{a|0}^{-1} \right) \\ &= \varepsilon + \lim_{c \rightarrow A^-} F_{1,a} \left( cp_{a|0}p_{a|0}^{-1} \right) - F_{1,a} \left( Ap_{a|0}p_{a|0}^{-1} \right) = \varepsilon. \quad (12) \end{aligned}$$

Therefore, by monotonicity,  $F_{1,b} \left( zp_{b|0}p_{b|1}^{-1} \right) - F_{1,a} \left( Ap_{a|0}p_{a|0}^{-1} \right) = \varepsilon$  for any  $z \in [G, g(A)]$  and  $\left( 1 - F_{0,a}(Ap_{a|0}p_{a|1}^{-1}) \right) p_{a|0} + \left( 1 - F_{0,b}(zp_{b|0}p_{b|1}^{-1}) \right) p_{b|0} = \alpha$  for any  $z \in [f(A), F]$ . Since  $A \in \mathcal{A}^+$ ,  $g(A) \geq f(A)$ . Additionally,  $F \geq G$ . Then,  $[G, g(A)] \cap [f(A), F] \neq \emptyset$ . Let

$A'$  be an element in this intersection. One can show  $A' \leq F \leq f(c_\alpha) \leq c_\alpha < A$  and  $A' \geq G \geq g(c_\alpha) > 0$ . Taking  $C = A$  and  $C' = A'$ , we have  $C > C' > 0$  and constraints (8) and (9) are satisfied.  $\square$

**Lemma S.3.** *If  $f(c_\alpha) > g(c_\alpha)$  and  $A = V$ , there exist  $C > C' > 0$  that satisfy equation 8 and 9.*

*Proof.* Let  $G$  and  $F$  be defined as in the proof of Lemma S.2. Then, similar to equation (12), we have  $F_{1,b} \left( G p_{b|0} p_{b|1}^{-1} \right) - F_{1,a} \left( V p_{a|0} p_{a|0}^{-1} \right) = \varepsilon$ . Then, for every  $z \in [G, \infty)$ ,

$$F_{1,b} \left( z p_{b|0} p_{b|1}^{-1} \right) - F_{1,a} \left( V p_{a|0} p_{a|0}^{-1} \right) = \varepsilon,$$

as  $F_{1,a} \left( V p_{a|0} p_{a|0}^{-1} \right) = 1 - \varepsilon$ . Furthermore, similar to equation (11)

$$\left( 1 - F_{0,a}(V p_{a|0} p_{a|1}^{-1}) \right) p_{a|0} + \left( 1 - F_{0,b}(F p_{b|0} p_{b|1}^{-1}) \right) p_{b|0} = \alpha,$$

and  $0 < G \leq F$ . Then, taking  $C = V$  and  $C' = F$  suffices as  $C = V > c_\alpha \geq f(c_\alpha) \geq F = C' \geq G > 0$ .  $\square$

**Lemma S.4.** *Conditional on  $\xi^a, t_{(k_*^{0,a})}^{0,a}$  and  $T$ ,  $R_1^a$  is equal in distribution to  $G_a + (1 - G_a) B_a$ . Furthermore,  $B_a$  is independent of  $\xi^a, t_{(k_*^{0,a})}^{0,a}$  and  $G_a$ .*

*Proof.* For all  $\mathcal{T}^{1,a} = \{t_1^{1,a}, t_2^{1,a}, \dots, t_{n_a^1}^{1,a}\}$  and  $j = 1, 2, \dots, n_a^1$ , let  $U_j = \mathbb{P}_{\text{left-out}} \left( T^a(X^{1,a}) \leq t_j^{1,a} \right)$ .

Then,  $U_j$ 's are independent random variables uniformly distributed on  $(0, 1)$ . To see this, denote  $F^{1,a}(z) = \mathbb{P}_{\text{left-out}} \left( T^a(X^{1,a}) \leq z \right)$ , then, for any  $z \in (0, 1)$ ,

$$\mathbb{P}_{\text{left-out}} (U_j \leq z) = \mathbb{P}_{\text{left-out}} (F^{1,a}(t_j^{1,a}) \leq z)$$

$$= \mathbb{P}_{\text{left-out}} (t_j^{1,a} \leq (F^{1,a})^{-1}(z)) = F^{1,a}((F^{1,a})^{-1}(z)) = z,$$

and the independence is guaranteed by the independence of  $t_j^{1,a}$ 's. Moreover, for fixed  $t_{k_*}^{0,a}$ ,  $\xi_j^a = \mathbb{I}\{t_j^{1,a} \leq t_{k_*}^{0,a}\} = \mathbb{I}\{U_j \leq F^{1,a}(t_{k_*}^{0,a})\}$ . Then, conditional on  $t_{k_*}^{0,a}$ ,  $F^{1,a}$  and  $\xi^a$ , the assertion is given by Lemma S.5.  $\square$

**Lemma S.5.** *Let  $U_1, U_2, \dots, U_n$  be  $n$  independent random variables that are uniformly distributed over  $[0, 1]$  and  $\xi_j = \mathbb{I}\{U_j \leq c\}$  for every  $j = 1, 2, \dots, n$  an arbitrary deterministic constant  $c \in [0, 1]$ . Then, for any  $1 \leq p < q \leq n$  and  $0 \leq c \leq s \leq 1$ ,*

$$\mathbb{P} \left( U_{(q)} \leq s \mid \sum_{j=1}^n \xi_j = p \right) = \sum_{k=q-p}^{n-p} \binom{n-p}{k} \frac{(s-c)^k (1-s)^{n-p-k}}{(1-c)^{n-p}}.$$

*That is,  $U_{(j)} \mid \left\{ \sum_{j=1}^n \xi_j = q \right\}$  is equal in distribution to  $c + (1-c)B$  where  $B$  is Beta distributed with parameters  $q-p$  and  $n-q+1$ .*

*Proof.* Note that

$$\mathbb{P} \left( U_{(q)} \leq s \mid \sum_{j=1}^n \xi_j = p \right) = \frac{\mathbb{P} (U_{(p)} \leq c < U_{(p+1)} \leq U_{(q)} \leq s)}{\mathbb{P} \left( \sum_{j=1}^n \xi_j = p \right)}.$$

The probability on the numerator equals

$$\binom{n}{p} c^p \sum_{k=q-p}^{n-p} \binom{n-p}{k} (s-c)^k (1-s)^{n-p-k},$$

whereas the probability of the denominator is

$$\binom{n}{p} c^p (1-c)^{n-p}.$$

Then, elementary algebra finishes the proof.  $\square$

**Lemma S.6.** *Let  $\{\mu\}_{n \geq 1}$  be an arbitrary sequence of numbers. Furthermore, let  $\{\sigma_n\}_{n \geq 1}$  and  $\{\varsigma_n\}_{n \geq 1}$  be two positive sequences such that  $|\sigma_n - \varsigma_n| \rightarrow 0$ , then*

$$\|\mathcal{N}(\mu_n, \sigma_n^2) - \mathcal{N}(\mu_n, \varsigma_n^2)\|_{TV} \rightarrow 0.$$

*Proof.* By Pinsker's inequality, it is sufficient to show the convergence of the Kulbeck-Leibler divergence of the two distributions. However, the Kulbeck-Leibler divergence of the two normal distributions  $D_{KL}(\mathcal{N}(\mu_n, \sigma_n^2) \parallel \mathcal{N}(\mu_n, \varsigma_n^2))$  in the assertion equals  $\frac{1}{2}(\log(\sigma_n^2/\varsigma_n^2) + \sigma_n^2/\varsigma_n^2 - 1)$  and converges to 0.  $\square$

**Lemma S.7.** *Let  $P$  and  $Q$  be two probability measures defined on  $(\Omega, \mathcal{F})$ . Assume, for some  $\varepsilon$ ,*

$$\sup_{B \in \mathcal{F}} |P(B) - Q(B)| \leq \varepsilon.$$

*Then, for any non-negative measurable function  $f$  bounded by a constant  $c$ ,*

$$|\mathbb{E}_P(f) - \mathbb{E}_Q(f)| \leq c\varepsilon.$$

*Proof.* Let  $g$  be an arbitrary positive step function defined on  $\Omega$  bounded by  $c$ , i.e.,

$$g(x) = \sum_{j=1}^n c_j \mathbb{I}\{x \in A_j\},$$

where  $A_j$ 's are disjoint sets in  $\mathcal{F}$ ,  $n$  is a constant and  $c_j \leq c$  for all  $1 \leq j \leq n$ . Let

$\mathcal{G}_p = \{A_j : P(A_j) \geq Q(A_j)\}$  and  $\mathcal{G}_q = \{A_j : P(A_j) < Q(A_j)\}$ . Then,

$$\begin{aligned}
|\mathbb{E}_P(g) - \mathbb{E}_Q(g)| &\leq \max_{\mathcal{G} \in \{\mathcal{G}_p, \mathcal{G}_q\}} \sum_{j \in \mathcal{G}} c_j (P(A_j) - Q(A_j)) \\
&\leq c \max_{\mathcal{G} \in \{\mathcal{G}_p, \mathcal{G}_q\}} \sum_{j \in \mathcal{G}} (P(A_j) - Q(A_j)) \\
&\leq c\varepsilon,
\end{aligned}$$

where the last inequality is given by the definition of total variation distance. Then, let

$\{f_m\}_{m \geq 1}$  be a sequence of increasing step functions that converge to  $f$  pointwise as  $m \rightarrow \infty$ .

Then,  $\mathbb{E}_P f_m \rightarrow \mathbb{E}_P f$  and  $\mathbb{E}_Q f_m \rightarrow \mathbb{E}_Q f$ . Thus,

$$\begin{aligned}
|\mathbb{E}_P(f) - \mathbb{E}_Q(f)| &\leq |\mathbb{E}_P(f) - \mathbb{E}_P f_m| + |\mathbb{E}_P(f_m) - \mathbb{E}_Q(f_m)| + |\mathbb{E}_Q(f) - \mathbb{E}_Q f_m| \\
&\leq |\mathbb{E}_P(f) - \mathbb{E}_P f_m| + c\varepsilon + |\mathbb{E}_Q(f) - \mathbb{E}_Q f_m|.
\end{aligned}$$

Letting  $m$  go to infinity on both sides of the inequality yields the result.  $\square$

**Lemma S.8.** *The equality in the distribution in (10) holds. Furthermore, the Beta distribution  $B_{p,q}$  is independent of the conditional distribution  $L_r^a$  in (10), regardless of their indices  $p, q$  and  $r$ .*

*Proof.* The first part of the proof follows the proof of Lemma S.5 Then, let a  $U_1, \dots, U_n$  be  $n$  independent uniform random variables and  $l_i = \sum_{j=1}^n \mathbb{I}\{U_j \leq c_i\}, i \in [m]$ , where  $c_1 \leq c_2 \leq \dots \leq c_m$  is a sequence of increasing constants. Furthermore, set  $c_0 = 0, c_{m+1} = 1, l_0 = 0$  and  $l_{m+1} = n$ . It suffices to show that  $U_{(q)} \mid \{l_1, l_2, \dots, l_m\}$  has a scaled and

shifted Beta distribution. That is, if  $l_i < q \leq l_{i+1}$  for any constant  $s$ ,

$$\mathbb{P}(U_{(q)} \leq s \mid l_1, l_2, \dots, l_m) = \sum_{j=q}^{l_{i+1}} \binom{l_{i+1} - l_i}{q - l_i} \left( \frac{s - c_i}{c_{i+1} - c_i} \right)^{q - l_i} \left( 1 - \frac{s - c_i}{c_{i+1} - c_i} \right)^{l_{i+1} - q}.$$

Indeed, one can write

$$\mathbb{P}(U_{(q)} \leq s \mid l_1, l_2, \dots, l_m) = \frac{\mathbb{P}(U_{(q)} \leq s, U_{(l_1)} \leq c_1 < U_{(l_1+1)} \leq \dots U_{(l_m-1)} \leq c_{m-1} < U_{(l_m)} \leq c_m)}{\mathbb{P}(U_{(l_1)} \leq c_1 < U_{(l_1+1)} \leq \dots U_{(l_m-1)} \leq c_{m-1} < U_{(l_m)} \leq c_m)}.$$

The denominator is a multinomial probability and thus equals

$$\binom{m+1}{l_1, l_2 - l_1, l_3 - l_2, \dots, n - l_m} c_1^{l_1} (c_2 - c_1)^{l_2 - l_1} \dots (1 - c_m)^{n - l_m}.$$

The numerator equals

$$\begin{aligned} \sum_{j=q}^{l_{i+1}} \binom{m+1}{l_1 - l_0, l_2 - l_1, \dots, j - l_i, l_{i+1} - j, \dots, l_{m+1} - l_m} (s - c_i)^{j - l_i} (c_{i+1} - s)^{l_{i+1} - j} \\ \times \prod_{k \in [m+1], k \neq i} (c_{k+1} - c_k)^{l_{k+1} - l_k}. \end{aligned}$$

Then, elementary algebra gives the desired result.  $\square$

**Lemma S.9.** *Let  $\{(T_j, S_j)\}_{j=1}^n$  be i.i.d. copies of the random couple  $(T, S) \in \mathbb{R} \times \{a, b\}$  and  $n_a = \sum_{j=1}^n \mathbb{1}\{S_j = a\}$ . Define  $\mathcal{A} = \{c_1 \leq n_a \leq c_2\}$  for deterministic constants  $c_1, c_2$ .*

*Then, for any  $\eta$ ,*

$$\mathbb{P} \left( \left\{ \sup_{c \in \mathbb{R}} \left| \frac{1}{n_a} \sum_{i: S_i = a} \mathbb{1}\{T_i > c\} - \mathbb{P}(T > c \mid S = a) \right| > \eta \right\} \cap \mathcal{A} \right) \leq 2e^{-\frac{1}{2}c_1\eta^2}.$$

*Proof.* Let  $\mathcal{I}_n^j = \{I \subset [n] : |I| = j\}$  be the collection of subsets of  $[n]$  that have cardinality  $j$ . Note that  $\mathcal{A} = \bigcup_{j=\lceil c_1 \rceil}^{\lfloor c_2 \rfloor} \bigcup_{I \in \mathcal{I}_n^j} \mathcal{A}_I$  where  $\mathcal{A}_I = \{S_i = a, \forall i \in I, \text{ and } S_i = b, \forall i \in [n] \setminus I\}$ . Thus,

$$\begin{aligned} & \mathbb{P} \left( \left\{ \sup_{c \in \mathbb{R}} \left| \frac{1}{n_a} \sum_{i: S_i = a} \mathbb{I}\{T_i > c\} - \mathbb{P}(T > c \mid S = a) \right| > \eta \right\} \cap \mathcal{A} \right) \\ &= \sum_{j=\lceil c_1 \rceil}^{\lfloor c_2 \rfloor} \sum_{I \in \mathcal{I}_n^j} \mathbb{P} \left( \left\{ \sup_{c \in \mathbb{R}} \left| \frac{1}{n_a} \sum_{i: S_i = a} \mathbb{I}\{T_i > c\} - \mathbb{P}(T > c \mid S = a) \right| > \eta \right\} \cap \mathcal{A}_I \right) \\ &= \sum_{j=\lceil c_1 \rceil}^{\lfloor c_2 \rfloor} \sum_{I \in \mathcal{I}_n^j} \mathbb{P} \left( \sup_{c \in \mathbb{R}} \left| \frac{1}{j} \sum_{i: S_i = a} \mathbb{I}\{T_i > c\} - \mathbb{P}(T > c \mid S = a) \right| > \eta \mid \mathcal{A}_I \right) \mathbb{P}(\mathcal{A}_I). \end{aligned}$$

It is easy to check that  $T_1, \dots, T_n$  are independent conditional on  $S_1, \dots, S_n$ . Therefore,

$$\mathbb{P} \left( \sup_{c \in \mathbb{R}} \left| \frac{1}{j} \sum_{i: S_i = a} \mathbb{I}\{T_i > c\} - \mathbb{P}(T > c \mid S = a) \right| > \eta \mid \mathcal{A}_I \right) \leq 2e^{-\frac{1}{2}j\eta^2},$$

by Dvoretzky–Kiefer–Wolfowitz inequality. Then,

$$\sum_{j=\lceil c_1 \rceil}^{\lfloor c_2 \rfloor} \sum_{I \in \mathcal{I}_n^j} 2e^{-\frac{1}{2}j\eta^2} \mathbb{P}(\mathcal{A}_I) \leq 2e^{-\frac{1}{2}c_1\eta^2} \sum_{j=\lceil c_1 \rceil}^{\lfloor c_2 \rfloor} \sum_{I \in \mathcal{I}_n^j} \mathbb{P}(\mathcal{A}_I) \leq 2e^{-\frac{1}{2}c_1\eta^2}.$$

□

## D Additional Numerical Results

### D.1 The Adult dataset

We utilize the widely studied Adult dataset [Becker and Kohavi, 1996], which comprises 48,842 instances. Each instance includes demographic information, job-related details, and

a binary categorical variable  $Y$  indicating whether an individual’s annual income exceeds 50,000 US dollars. This dataset is frequently employed in the machine learning fairness literature to assess algorithmic fairness in prediction tasks, where the objective is to predict  $Y$  using the remaining features. In such studies, the sensitive attribute is typically chosen as either “sex” or “race”. In this work, we designate “sex” as the sensitive attribute.

After the pre-processing steps borrowed from a popular Kaggle post<sup>5</sup>, the dataset is partitioned equally into training and testing subsets. Half of the training data are used to train a base algorithm, implemented as a single hidden layer neural network with 10 nodes in the hidden layer. The remaining half of the training data is utilized by the NP-EO<sub>OP</sub> and NP-EO<sub>MP</sub> algorithms to determine optimal thresholds. After training, the performance metrics  $R_0^a, R_1^a, R_0^b, R_1^b$  are computed on the testing dataset, along with  $R_0, R_1$ , and  $L_1$ . This entire procedure is repeated 1,000 times to approximate NP and EO violation rates. The parameters used in the analysis are set as follows:  $\alpha = 0.1$ ,  $\delta = 0.15$ ,  $\varepsilon = 0.15$ , and  $\gamma = 0.15$ .

The results presented in Table 1 convey three key findings. First, the classical algorithm fails to meet the predefined violation thresholds, as both the NP violation rate (0.234) and the EO violation rate (0.353) exceed the target levels of  $\varepsilon = \gamma = 0.15$ . Second, while the application of the NP method successfully reduces the NP violation rate to 0.132, which is below the target threshold, it leads to an increase in the EO violation rate (0.379). Finally, both proposed methods, NP-EO<sub>OP</sub> and NP-EO<sub>MP</sub> demonstrate their efficacy by effectively controlling both NP and EO violation rates. Notably, NP-EO<sub>MP</sub> achieves this without a substantial deterioration in the average type II error compared to the classical method,

---

<sup>5</sup>See <https://www.kaggle.com/code/yipfafa/r-income-prediction-with-knn-nn-decision-tree/report> for details

Table 1: Averages of type I errors, type II errors, and type II error disparities, along with violation rates of NP and EO constraints over 1,000 repetitions for the Adult dataset. Standard error of the means ( $\times 10^{-4}$ ) in parentheses

|                     | average of<br>type I errors | average of<br>type II errors | average of<br>type II error<br>disparities | NP violation<br>rate | EO violation<br>rate |
|---------------------|-----------------------------|------------------------------|--------------------------------------------|----------------------|----------------------|
| NP-EO <sub>OP</sub> | .084(6.22)                  | .462(34.79)                  | .106(13.59)                                | .038(60.49)          | .105(96.99)          |
| NP-EO <sub>MP</sub> | .089(6.54)                  | .424(37.34)                  | .099(13.59)                                | .156(114.80)         | .109(98.60)          |
| NP                  | .091(6.03)                  | .417(35.64)                  | .132(17.11)                                | .187(123.36)         | .379(153.49)         |
| classical           | .089(6.74)                  | .420(34.47)                  | .131(16.67)                                | .234(133.95)         | .353(151.20)         |

highlighting its ability to maintain predictive performance while ensuring fairness.

## D.2 Additional results from Simulation 1

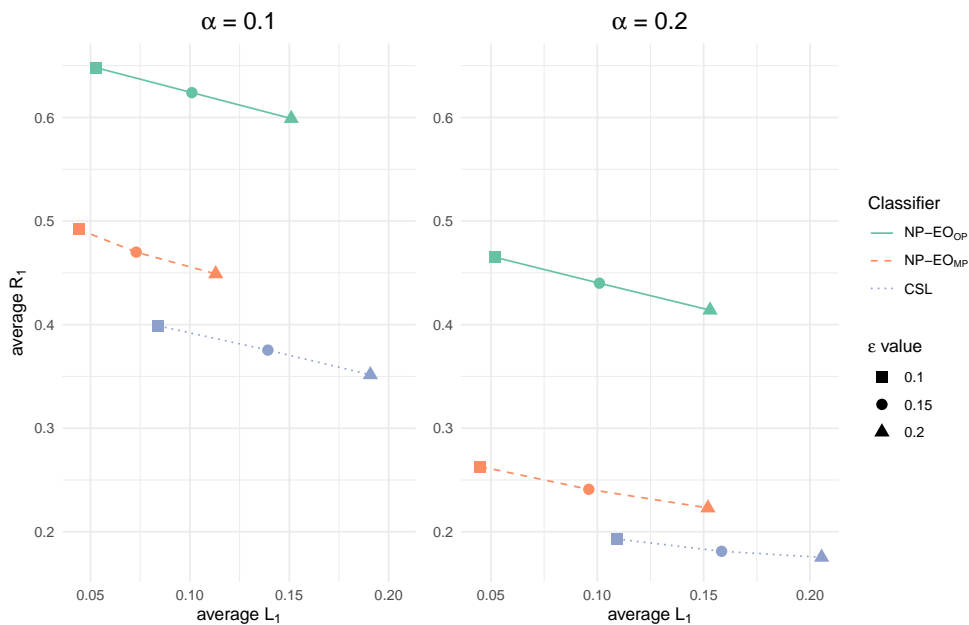

Figure 1: The performance of NP-EO<sub>OP</sub>, NP-EO<sub>MP</sub> and CSL across different  $\epsilon$  and  $\alpha$ .

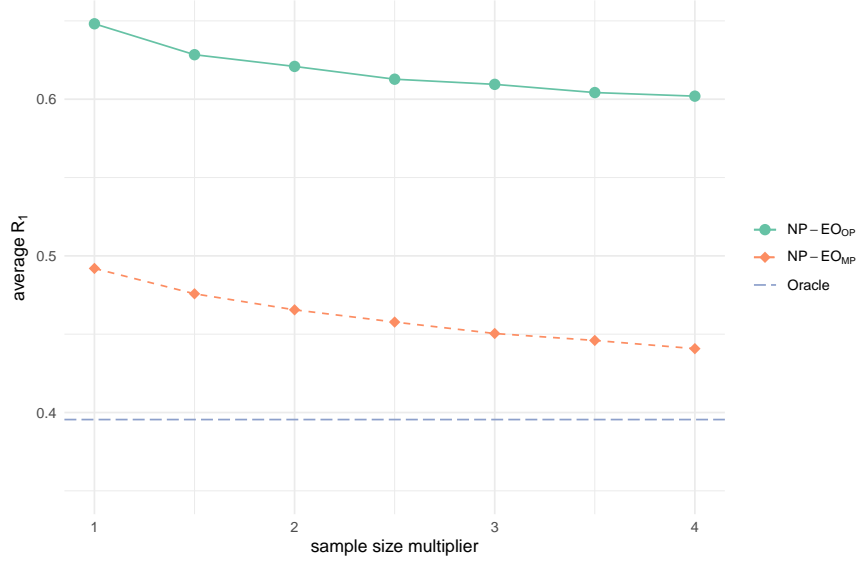

Figure 2: With parameters  $\alpha = 0.1$ ,  $\delta = 0.05$ ,  $\varepsilon = 0.1$ ,  $\gamma = 0.05$ , we report the behavior of the average type II errors as the sample size increases. In particular, the sample size multiplier indicates how many times the original sample size is increased from its initial setting used in Simulation 1.

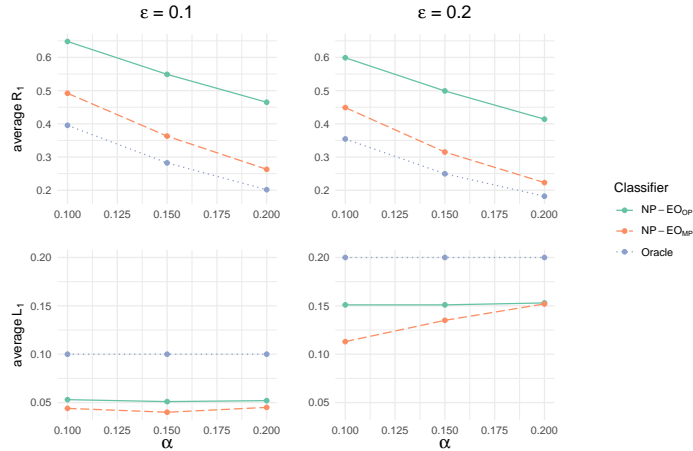

Figure 3: The performance of NP-EO<sub>OP</sub> and NP-EO<sub>MP</sub> across different combinations of  $\varepsilon$  and  $\alpha$ , as evaluated by the average  $R_1$  and  $L_1$

### D.3 Additional simulation

In this section, we provide an additional simulation study comparing NP-EO<sub>OP</sub> and NP-EO<sub>MP</sub> with the following methods: the classical algorithm, the NP umbrella algorithm, and the

NP umbrella algorithm mixed with random guesses.

The NP umbrella algorithm mixed with random guesses, inspired by Hardt et al. [2016], works as follows. We start with an NP classifier,  $\hat{\phi}_{\text{NP}}$ , trained by the NP umbrella algorithm. Without loss of generality, we assume  $R_1^a(\hat{\phi}_{\text{NP}}) > R_1^b(\hat{\phi}_{\text{NP}})$ . A naive method to make the EO constraint satisfied is to increase type II error for  $S = b$  by adding noise via a random guess classifier  $\phi_{\text{RG}}$  with  $\mathbb{P}(\phi_{\text{RG}} = 1) = \alpha$ . Then, for observation in the testing sample with  $S = a$ , we use  $\hat{\phi}_{\text{NP}}$  only; for observation with  $S = b$ , with probability  $p$ ,  $\hat{\phi}_{\text{NP}}$  is selected to classify this observation, and with probability  $1 - p$ ,  $\phi_{\text{RG}}$  is used. Note that  $R_1^b(\phi_{\text{RG}}) = 1 - \alpha$ . Then, for this mixed classifier  $\hat{\phi}_{\text{mixed}}$ ,  $R_1^a(\hat{\phi}_{\text{mixed}}) = R_1^a(\hat{\phi}_{\text{NP}})$  and  $R_1^b(\hat{\phi}_{\text{mixed}}) = pR_1^b(\hat{\phi}_{\text{NP}}) + (1 - p)(1 - \alpha)$ . As long as  $\hat{\phi}_{\text{NP}}$  is more powerful than  $\phi_{\text{RG}}$  on group  $a$ , i.e.,  $R_1^a(\hat{\phi}_{\text{NP}}) \leq 1 - \alpha$ ,  $\hat{\phi}_{\text{mixed}}$  can achieve EO by choosing  $p$  properly.

In particular, we choose the probability  $p$  by 20-fold cross validation: we train an NP classifier on 19 folds of the training data and compute the estimated  $R_1^a(\hat{\phi}_{\text{NP}})$  and  $R_1^b(\hat{\phi}_{\text{NP}})$  on the left-out fold. Since  $R_1^a(\phi_{\text{RG}})$  and  $R_1^b(\phi_{\text{RG}})$  are explicit, we can directly estimate  $R_1^a(\hat{\phi}_{\text{mixed}})$ ,  $R_1^b(\hat{\phi}_{\text{mixed}})$  and thus type II error disparity for every value of  $p$  and the option of adding random guesses for either  $S = a$  or  $S = b$ . We traverse all the combinations of  $p = 0, 0.1, 0.2, 0.3, \dots, 0.9$  and the options of adding random guesses to both  $S$  components. Next, for every combination, we calculate the estimated type II error disparity for every fold and thus compute the estimated probability of type II error disparity exceeding  $\varepsilon$ . Finally, we select the combination such that this estimated probability is smaller than or equal to  $\gamma$ . If there are multiple such combinations, we select the one with the largest  $p$ . Then the resulting  $\hat{\phi}_{\text{mixed}}$  satisfies high-probability NP and EO constraints.

**Simulation S.1.** Let  $X^{y,s}$  be uniformly distributed in a three-dimensional ball  $B_{y,s}$  with

Table 2: Averages of type I/II errors, along with violation rates of NP and EO constraints over 1,000 repetitions for Simulation S.1. Standard error of the means ( $\times 10^{-4}$ ) in parentheses

|                               | average of<br>type I errors | average of<br>type II errors | average of<br>type II error<br>disparities | NP violation<br>rate | EO violation<br>rate |
|-------------------------------|-----------------------------|------------------------------|--------------------------------------------|----------------------|----------------------|
| NP-EO <sub>OP</sub>           | .012(1.11)                  | .478(12.50)                  | .134(12.44)                                | 0(0)                 | .045(65.59)          |
| NP-EO <sub>MP</sub>           | .037(1.88)                  | .348(13.81)                  | .139(12.88)                                | .018(42.06)          | .074(82.82)          |
| NP mixed with<br>random guess | .040(1.24)                  | .580(14.64)                  | .040(10.07)                                | .012(34.45)          | 0(0)                 |
| NP                            | .039(1.91)                  | .168(3.81)                   | .398(6.56)                                 | .041(63.74)          | 1(0)                 |
| classical                     | .094(1.80)                  | .096(1.32)                   | .341(6.32)                                 | 1(0)                 | 1(0)                 |

radius 1 and centered at  $O_{y,s}$ , where  $O_{0,a} = (0, 0, 0)^\top$ ,  $O_{1,a} = (1, 0, -1)^\top$ ,  $O_{0,b} = (1, 1, 1)^\top$  and  $O_{1,b} = (-1, 1, 0)^\top$ . Furthermore,  $n^{0,a} = 800$ ,  $n^{1,a} = 400$ ,  $n^{0,b} = 1200$  and  $n^{1,b} = 1600$ . We also set  $\alpha = 0.05$ ,  $\delta = 0.05$ ,  $\varepsilon = 0.2$  and  $\gamma = 0.05$ . The base algorithm used is logistic regression. The numerical results associated with this simulation are reported in Table 2.

In this simulation, the classical classifier admits the lowest type II error; the NP classifier comes in second place. This is not surprising as the NP paradigm controls the type I error to a low level with high probability, thereby resulting in a higher type II error. The NP and EO violation rates are both higher than the target levels for the classical classifier, whereas the NP classifier fails to keep the EO violation rate under the target level. These two classifiers adopt no design for EO adjustments; thus, it is expected that the EO requirement will fail.

The remaining three algorithms, NP-EO<sub>OP</sub>, NP-EO<sub>MP</sub> and NP mixed with random guesses, are built to achieve the high-probability NP and EO constraints. All three algorithms produce an overall type II error larger than that of the NP paradigm. This is the price paid for equality in our classification algorithms. For reference, we remark that the “nearly trivial” NP-EO classifier, a random guess that returns 1 with probability 0.05 and 0 otherwise, has an overall type II error as high as 0.95. Benchmarked against this result,

the classifiers listed in Table 2 have much smaller type II errors. Moreover, in terms of the overall type II error, it is clear that NP-EO<sub>OP</sub> and NP-EO<sub>MP</sub> outperform NP mixed with random guesses, suggesting the effectiveness of our proposed algorithms. Between the two proposed algorithms, NP-EO<sub>MP</sub> yields a larger average overall type I error and type I error violation rate, and smaller overall type II error than NP-EO<sub>OP</sub>, which agrees with the argument in Section 4.2 that NP-EO<sub>MP</sub> uses multiple pivots to select thresholds more effectively. In conclusion, the two simulation studies illustrate that our proposed algorithms under the NP-EO paradigm can achieve the goals of regulating equality of opportunities and controlling the type I error while only paying a modest price in terms of the less consequential type II error.

## E Algorithms

In this section, we present the supplementary algorithms in this work.

## References

- Xin Tong, Yang Feng, and Jingyi Jessica Li. Neyman-pearson classification algorithms and np receiver operating characteristics. *Science Advances*, 4(2):eaao1659, 2018.
- J. Ghosh and R. Ramamoorthi. Bayesian nonparametrics. *Springer Series in Statistics*, 16, 01 2011.
- E.L. Lehmann and J.P Ramano. *Testing Statistical Hypotheses*. Springer, 2005.

---

**Algorithm 3:** EO violation algorithm

---

**Input** :  $l_a, l_b, n_a, n_b$  : constants such that  $l_a \leq n_a$  and  $l_b \leq n_b$   
 $\varepsilon$ : upper bound for the type II error disparity  
 $\gamma$ : type II error disparity violation rate target

```
1  $\hat{\gamma} \leftarrow 1$ 
2  $\hat{R}_1 \leftarrow 1$ 
3  $k_a^* \leftarrow n_a^1$ 
4  $k_b^* \leftarrow n_b^1$ 
5 for  $i = l_a + 1, l_a + 2, \dots, n_a^1$  do
6   for  $j = l_b + 1, l_b + 2, \dots, n_b^1$  do
7     /* Estimating  $\mathbb{P}(|F^{1,a}(i) - F^{1,b}(j)| > \varepsilon)$  in (10) by Monte-Carlo simulation */
8      $K \leftarrow 1000$ ; //  $K$  is the number of copies of  $F^{1,a}(i)$  and  $F^{1,b}(j)$  generated. It is set to 1000 in all numerical experiments in this work.
9     for  $k = 1, 2, \dots, K$  do
10       $G_k^a \leftarrow \mathcal{N}\left(l_a/n_a^1, \frac{(l_a/n_a^1)((1-l_a)/n_a^1)}{n_a^1}\right)$ 
11       $G_k^b \leftarrow \mathcal{N}\left(l_b/n_b^1, \frac{(l_b/n_b^1)((1-l_b)/n_b^1)}{n_b^1}\right)$ 
12       $B_k^a \leftarrow \text{Beta}(i - l_a, n_a - i + 1)$ 
13       $B_k^b \leftarrow \text{Beta}(j - l_b, n_b - j + 1)$ ; //  $B_k^a, B_k^b$  are two Beta distributed random variables
14       $F_k^a \leftarrow G_k^a + (1 - G_k^a)B_k^a$ 
15       $F_k^b \leftarrow G_k^b + (1 - G_k^b)B_k^b$ 
16    end
17     $\hat{\gamma} \leftarrow \frac{1}{K} \sum_{k=1}^K \mathbb{I}\{|F_k^a - F_k^b| > \varepsilon\}$ 
18     $\hat{R}_1^{\text{new}} \leftarrow \frac{(i-1)+(j-1)}{n_a+n_b}$ 
19    if  $\hat{\gamma} \leq \gamma$  and  $\hat{R}_1^{\text{new}} < \hat{R}_1$  then
20       $k_a^* \leftarrow i$ 
21       $k_b^* \leftarrow j$ 
22       $\hat{R}_1 \leftarrow \hat{R}_1^{\text{new}}$ 
23    end
24  end
25 end
Output:  $(k_a^*, k_b^*)$ 
```

---

Christophe Denis, Romuald Elie, Mohamed Hebiri, and François Hu. Fairness guarantees in multi-class classification with demographic parity. *JMLR*, 25(130):1–46, 2024.

L Elisa Celis, Lingxiao Huang, Vijay Keswani, and Nisheeth K Vishnoi. Classification with fairness constraints: A meta-algorithm with provable guarantees. In *FAccT*, pages

319–328, 2019.

Equal Employment Opportunity Commission et al. Uniform guidelines on employee selection procedures. *Fed Register*, 44, 1979.

Aditya Krishna Menon and Robert C Williamson. The cost of fairness in binary classification. In *FAccT*, pages 107–118. PMLR, 2018.

Harry Holzer and David Neumark. Assessing affirmative action. *J. Econ. Lit.*, 38(3):483–568, 2000.

Brian W Collins. Tackling unconscious bias in hiring practices: The plight of the rooney rule. *NYUL Rev.*, 82:870, 2007.

Barry Becker and Ronny Kohavi. Adult. UCI Machine Learning Repository, 1996. DOI: <https://doi.org/10.24432/C5XW20>.

Moritz Hardt, Eric Price, and Nati Srebro. Equality of opportunity in supervised learning. In *NeurIPS*, pages 3315–3323, 2016.

---

**Algorithm 4:** Adjusted EO violation algorithm

---

**Input** :  $k(a), k(b)$ : orders of possible thresholds  
           $n_a^0, n_b^0, n_a^1, n_b^1$ : sample sizes  
           $l_a(1), l_a(2), \dots, l_a(n_a^0), l_b(1), l_b(2), \dots, l_b(n_b^0)$ : integers such that  
           $0 \leq l_a(1) \leq l_a(2) \leq \dots \leq l_a(n_a^0) \leq n_a^1$  and  $0 \leq l_b(1) \leq l_b(2) \leq \dots \leq l_b(n_b^0) \leq n_b^1$   
           $\varepsilon$ : upper bound for the type II error disparity

```
1 for  $s = a, b$  do
2    $l_s(0) \leftarrow 0$ 
3    $l_s(n_s^0 + 1) \leftarrow n_s^1$ 
   /* Specifying parameters for the Gaussian distribution by
   Bernstein-von Mises theorem */
4    $d_s(j) \leftarrow l_s(j) - l_s(j - 1), j \in [n_s^0 + 1]$ 
5    $\mu^s \leftarrow \left( \frac{d_s(1)}{n_s^1}, \frac{d_s(2)}{n_s^1}, \dots, \frac{d_s(n_s^0 + 1)}{n_s^1} \right)^\top$  ; //  $\mu^s$  is the mean vector for
   multivariate normal
6    $\Sigma^s \leftarrow$ 
      
$$\begin{bmatrix} \frac{(d_s(1)/n_s^1)(1-d_s(1)/n_s^1)}{n_s^1} & -\frac{(d_s(1)/n_s^1)(d_s(2)/n_s^1)}{n_s^1} & \dots & -\frac{(d_s(1)/n_s^1)(d_s(n_s^0+1)/n_s^1)}{n_s^1} \\ -\frac{(d_s(2)/n_s^1)(d_s(1)/n_s^1)}{n_s^1} & \frac{(d_s(2)/n_s^1)(1-d_s(2)/n_s^1)}{n_s^1} & \dots & -\frac{(d_s(2)/n_s^1)(d_s(n_s^0+1)/n_s^1)}{n_s^1} \\ \vdots & \vdots & \ddots & \vdots \\ -\frac{(d_s(n_s^0+1)/n_s^1)(d_s(1)/n_s^1)}{n_s^1} & -\frac{(d_s(n_s^0+1)/n_s^1)(d_s(2)/n_s^1)}{n_s^1} & \dots & \frac{(d_s(n_s^0+1)/n_s^1)(1-d_s(n_s^0+1)/n_s^1)}{n_s^1} \end{bmatrix}$$

   ; //  $\Sigma^s$  is the covariance matrix
   /* Specifying parameters for Beta distribution */
7    $k_s \leftarrow \max\{j \in [n_s^0 + 1] : l_s(j) < k(s)\}$ 
8    $k_l^s \leftarrow l_s(k_s)$ 
9    $k_u^s \leftarrow l_s(k_s + 1)$ 
10   $K \leftarrow 1000$ 
11  for  $h = 1, 2, \dots, K$  do
12     $W_h^s \leftarrow \mathcal{N}(\mu^s, \Sigma^s)$  ; //  $W_h^s$  is a  $(n_s^0 + 1)$ -dimensional Gaussian vector
13     $B_h^s = \text{Beta}(k(s) - k_l^s, k_u^s - k(s) + 1)$ 
14    if  $k_s = 0$  then
15       $Z_h^s = [W_h^s]_1$  ; //  $[W_h^s]_j$  is the  $j^{\text{th}}$  element of  $W_h^s$ 
16       $V_h^s = Z_h^s B_h^s$ 
17    else if  $k_s = n_s^0$  then
18       $Z_h^s = \sum_{j=1}^{n_s^0} [W_h^s]_j$ 
19       $V_h^s = Z_h^s + (1 - Z_h^s) B_h^s$ 
20    else
21       $Z_h^s = \sum_{j=1}^{k_s} [W_h^s]_j$ 
22       $V_h^s = Z_h^s + [W_h^s]_{k_s+1} B_h^s$ 
23    end
24  end
25 end
26  $v_a = \frac{1}{K} \sum_{h=1}^K \mathbb{I}\{V_h^a - V_h^b > \varepsilon\}$ 
27  $v_b = \frac{1}{K} \sum_{h=1}^K \mathbb{I}\{V_h^b - V_h^a > \varepsilon\}$  ; //  $v_a, v_b$  are one-sided violation rate
Output:  $(v_a, v_b)$ 
```

---

---

**Algorithm 5:** Order selection algorithm

---

**Input** :  $k_a, k_b$ : starting pivots  
           $n_a^0, n_b^0, n_a^1, n_b^1$ : sample sizes  
           $l_a(1), l_a(2), \dots, l_a(n_a^0), l_b(1), l_b(2), \dots, l_b(n_b^0)$ : two increasing sequences  
           $\varepsilon$ : upper bound for the type II error disparity  
           $\gamma$ : type II error disparity violation rate target

```
1  $l_s(0) \leftarrow 0$  for  $s \in \{a, b\}$ 
2  $l_s(n_s^0 + 1) \leftarrow n_s^1$  for  $s \in \{a, b\}$ 
3  $k(s) \leftarrow l_s(k_s) + 1$  for  $k \in \{a, b\}$ 
4 while TRUE do
5    $(v_a, v_b) \leftarrow \text{Adjusted EO violation algorithm}(k(s), n_s^y, l_s(1), \dots, l_s(n_s^0), \varepsilon)$ 
     for  $s \in \{a, b\}$  and  $y \in \{0, 1\}$ 
6   if  $v_a > \gamma$  and  $v_b > \gamma$  then
7      $k_s \leftarrow k_s + 1$  for  $s \in \{a, b\}$ 
8      $k(s) \leftarrow l_s(k_s) + 1$  for  $k \in \{a, b\}$ 
9   else if  $v_a > \gamma$  then
10    if  $k_a = 0$  or  $k_b = n_b^0$  then
11       $k(b) \leftarrow k(b) + 1$ 
12    else
13       $k_a^{\text{new}} \leftarrow k_a^{\text{new}} - 1$ 
14       $k_b^{\text{new}} \leftarrow k_b^{\text{new}} + 1$ 
15       $k^{\text{new}}(s) \leftarrow l_s(k_s) + 1$  for  $k \in \{a, b\}$ 
16       $(v_a^{\text{new}}, v_b^{\text{new}}) \leftarrow$ 
        Adjusted EO violation algorithm $(k^{\text{new}}(s), n_s^y, l_s(1), \dots, l_s(n_s^0), \varepsilon)$ 
        for  $s \in \{a, b\}$  and  $y \in \{0, 1\}$ 
17      if  $v_b^{\text{new}} \leq \gamma$  then
18         $k_s = k_s^{\text{new}}$  for  $s \in \{a, b\}$ 
19         $k(s) \leftarrow k^{\text{new}}(s)$  for  $s \in \{a, b\}$ 
20      else
21         $k(b) \leftarrow k(b) + 1$ 
22      end
23    end
24   else if  $v_b > \gamma$  then
25     do Step 10 - 22 with  $a$  and  $b$  switched
26   else
27     Output:  $(k_a, k_b)$ 
28 end
```

---
